# Supplementary material for: Nonlinear $\sigma$-model for disordered systems with intrinsic spin-orbit coupling
Source: arXiv:2205.14075 ancillary file (2022-05-27)
Supplement: Supplementary file 1 [file gradexp-out.pdf]

# Intrinsic spin-Hall effect in a nonlinear $\sigma$-model: Supplementary Material

P. Virtanen

*Department of Physics and Nanoscience Center,*
*University of Jyväskylä,*
*P.O. Box 35 (YFL),*
*FI-40014 University of Jyväskylä,*
*Finland*

F. S. Bergeret

*Centro de Física de Materiales (CFM-MPC) Centro Mixto CSIC-UPV/EHU,*
*E-20018 Donostia-San Sebastián,*
*Spain*
*Donostia International Physics Center (DIPC),*
*20018 Donostia–San Sebastián,*
*Spain*

I. V. Tokatly

*Nano-Bio Spectroscopy Group,*
*Departamento de Polímeros y Materiales Avanzados: Física,*
*Química y Tecnología,*
*Universidad del País Vasco (UPV/EHU),*
*20018 Donostia-San Sebastián,*
*Spain*
*IKERBASQUE, Basque Foundation for Science, 48011 Bilbao,*
*Spain*
*Donostia International Physics Center (DIPC),*
*20018 Donostia-San Sebastián,*
*Spain*
*ITMO University,*
*Department of Physics and Engineering,*
*Saint-Petersburg,*
*Russia*

(Dated: May 13, 2022)

```
This Supplementary Material package contains the following files:

- gradexp.sage: Implementation of the gradient expansion discussed in
  the main text, using SageMath (version 9.4).

  You can run it with ‘sage gradexp.sage‘ and it will print results
  in text notation, and LaTeX.

- gradexp.tex: Source file for generating gradexp.sage, using
  SageTeX. Contains instructions and detailed explanations.

- gradexp.pdf: PDF version of the above, with results embedded.

- Makefile.gradexp: Makefile for re-generating output files.
```

## CONTENTS


I. gradexp.tex 2

II. Momentum integrals 2

III. Gradient expansion 3
- A. Basic algebra and index notation 3
- B. Natural units 6
- C. Momentum direction average 6
  - 1. Wigner convolution product 8
- D. Momentum integration and $p_F\ell$ expansion 10
- E. Tr ln expansion 11
- F. Trace permutation and integration by parts 13
- G. Covariant form 15
- H. Next orders in $p_F\ell$ 18
- I. Symmetrization 18
- J. Expansion with $a_0$ 20

IV. Longitudinal shift 23
- A. Computer algebra 23

V. Saddle-point equations 28
- A. Matrix current 29

A. Indexed letter monoid 30


## I. GRADEXP.TEX

This file contains the implementation of gradient expansion in NLsM with gauge fields. It is written for the main part in literate programming style, using *SageMath* 9.4, and *SageTeX*, and contains both code listings and typeset results.

You can run this file `.sage` file with commands:

```
pdflatex gradexp.tex
sage gradexp.sagetex.sage
pdflatex gradexp.tex
pdflatex gradexp.tex
sagetex-extract --no-inline -o gradexp.sage gradexp.tex
```

The `sage` command will print the results in text and LaTeX format, in addition to generating input files for the rest of the latex commands.

## II. MOMENTUM INTEGRALS

Define first a function evaluating the constants $C_{\beta N n}$ appearing in the momentum integrals:

**Code 1** (Evaluation of $\tilde{C}(\beta, N, n)$.).

```
def C_tilde(beta, N, n, exact=False, order=0, ndim=3, regularize=True):
    psi, z = SR.var('psi z')
    assert beta in NN

    is_convergent = (beta + ndim/2 < N + n)

    if not (is_convergent or regularize):
        # Return symbolic value for nonconvergent case, if not going to regularize
        return SR.var('C_{}{}{}'.format(beta, N, n)), is_convergent

    if ndim % 2 == 0:
```

TABLE I Values for $\tilde{C}(\beta, N, n)$, expanded in $\psi = p_F \ell \gg 1$ up to $\mathcal{O}(\psi^0)$, for $d = 2$. Regularized non-converging values are shown as $\sim \ldots$ (in red).

| $\beta$, $N$ | $n=0$ | $n=1$ | $n=2$ | $n=3$ | $n=4$ |
|---|---|---|---|---|---|
| 0, 1 | $\infty$ | 1 | - | - | - |
| 0, 2 | $\frac{i\psi}{2} - \frac{i}{\pi}$ | 0 | $-\frac{i\psi}{2}$ | - | - |
| 0, 3 | $-\frac{i}{2\pi}$ | $\frac{\psi^2}{8}$ | 0 | $-\frac{3\psi^2}{8}$ | - |
| 0, 4 | $\frac{i\psi^3}{16} - \frac{i}{3\pi}$ | 0 | $-\frac{i\psi^3}{16}$ | 0 | $\frac{5i\psi^3}{16}$ |
| 1, 1 | $\infty$ | $\infty$ | - | - | - |
| 1, 2 | $\infty$ | $-\frac{1}{2}$ | $-\frac{i\psi}{2}$ | - | - |
| 1, 3 | $-\frac{3i\psi}{8} + \frac{i}{2\pi}$ | $\frac{\psi^2}{8}$ | $\frac{i\psi}{8}$ | $-\frac{3\psi^2}{8}$ | - |
| 1, 4 | $\frac{i\psi^3}{16} + \frac{i}{6\pi}$ | $-\frac{\psi^2}{16}$ | $-\frac{i\psi^3}{16}$ | $\frac{\psi^2}{16}$ | $\frac{5i\psi^3}{16}$ |
| 2, 1 | $\infty$ | $\infty$ | - | - | - |
| 2, 2 | $\infty$ | $\infty$ | $-\frac{i\psi}{2}$ | - | - |
| 2, 3 | $\infty$ | $\frac{\psi^2}{8} + \frac{3}{8}$ | $\frac{i\psi}{4}$ | $-\frac{3\psi^2}{8} - \frac{1}{8}$ | - |
| 2, 4 | $\frac{i\psi^3}{16} + \frac{5i\psi}{16} - \frac{i}{3\pi}$ | $-\frac{\psi^2}{8}$ | $-\frac{i\psi^3}{16} - \frac{i\psi}{16}$ | $\frac{\psi^2}{8}$ | $\frac{5i\psi^3}{16} + \frac{i\psi}{16}$ |

```
        # Fix branch for log(-1 - z) explicitly, for regular taylor expansion at z -> i0^+
        pre = {1: I/(2*pi) * (log(1 + z) - I*pi),
               -1: I/(2*pi) * (log(1 + z) + I*pi)}
        d_half = ndim/2
    else:
        # sqrt(-1 - z)
        pre = {1: I/2 * (-I * sqrt(1 + z)),
               -1: I/2 * (I * sqrt(1 + z))}
        d_half = (ndim-1)/2

    if not exact:
        # Expand first, to ensure we stay in the right branch
        pre = {k: v.taylor(z, 0, 2*N + max(0, order)) for k, v in pre.items()}

    f = I**(n+1) * (-1)**N / pi * psi**(-n) * (1+z)**(beta+d_half-1) * z**(N-n) / (z**2 + psi**-2)**N
    r = sum(2 * I * pi * (f*pre[s]).residue(z==s*I/psi) for s in (-1, 1))
    if exact:
        return r, is_convergent
    return r.taylor(psi, oo, order).expand(), is_convergent
```

We tabulate them in Tables I and II.

## III. GRADIENT EXPANSION

### A. Basic algebra and index notation

This will be done using *SageMath*, and SageTeX (so the various expressions below are not written manually in this TeX file, and the complete source code is shown here).

First, define the variables and their algebra. We'll deal with monomials formed from $\delta_{ij}$, $a_{k\ldots}$, $\Lambda$, $\mathcal{G}$, $F_{ij}$ and $\Lambda_{\ldots}$ of which only the first is commutative. Collapsing indices when multiplying by $\delta_{ij}$, index permutation symmetries, and $\Lambda^2 = Q^2 = 1$ are handled on the monomial level. (Any summation convention is not assumed yet.) We'll also define some ordering for the monomials. Because we are using an index notation with potentially arbitrary many indices and want to do manipulations on them, it's easiest to define a custom semigroup/monoid for the monomials and build algebra on that. See Appendix A for the code listing of `indexed_letter_monoid.py`.

TABLE II Values for $\tilde{C}(\beta, N, n)$, expanded in $\psi = p_F\ell \gg 1$ up to $\mathcal{O}(\psi^0)$, for $d = 3$. Regularized non-converging values are shown as $\sim (\ldots)$ (in red).

| $\beta$, $N$ | $n=0$ | $n=1$ | $n=2$ | $n=3$ | $n=4$ |
|---|---|---|---|---|---|
| 0, 1 | $\infty$ | 1 | - | - | - |
| 0, 2 | $\frac{i\psi}{2}$ | $-\frac{1}{4}$ | $-\frac{i\psi}{2}$ | - | - |
| 0, 3 | $-\frac{3i\psi}{16}$ | $\frac{\psi^2}{8} - \frac{3}{64}$ | $\frac{i\psi}{16}$ | $-\frac{3\psi^2}{8} + \frac{1}{64}$ | - |
| 0, 4 | $\frac{i\psi^3}{16} - \frac{5i\psi}{128}$ | $-\frac{\psi^2}{32} - \frac{5}{256}$ | $-\frac{i\psi^3}{16} + \frac{i\psi}{128}$ | $\frac{\psi^2}{32} + \frac{1}{256}$ | $\frac{5i\psi^3}{16} - \frac{i\psi}{128}$ |
| 1, 1 | $\infty$ | $\infty$ | - | - | - |
| 1, 2 | $\infty$ | $-\frac{3}{4}$ | $-\frac{i\psi}{2}$ | - | - |
| 1, 3 | $-\frac{9i\psi}{16}$ | $\frac{\psi^2}{8} + \frac{9}{64}$ | $\frac{3i\psi}{16}$ | $-\frac{3\psi^2}{8} - \frac{3}{64}$ | - |
| 1, 4 | $\frac{i\psi^3}{16} + \frac{15i\psi}{128}$ | $-\frac{3\psi^2}{32} + \frac{5}{256}$ | $-\frac{i\psi^3}{16} - \frac{3i\psi}{128}$ | $\frac{3\psi^2}{32} - \frac{1}{256}$ | $\frac{5i\psi^3}{16} + \frac{3i\psi}{128}$ |
| 2, 1 | $\infty$ | $\infty$ | - | - | - |
| 2, 2 | $\infty$ | $\infty$ | $-\frac{i\psi}{2}$ | - | - |
| 2, 3 | $\infty$ | $\frac{\psi^2}{8} + \frac{45}{64}$ | $\frac{5i\psi}{16}$ | $-\frac{3\psi^2}{8} - \frac{15}{64}$ | - |
| 2, 4 | $\frac{i\psi^3}{16} + \frac{75i\psi}{128}$ | $-\frac{5\psi^2}{32} - \frac{25}{256}$ | $-\frac{i\psi^3}{16} - \frac{15i\psi}{128}$ | $\frac{5\psi^2}{32} + \frac{5}{256}$ | $\frac{5i\psi^3}{16} + \frac{15i\psi}{128}$ |

**Code 2** (Algebra definition).

```
from indexed_letter_monoid import IndexedLetterMonoid

dummy_idxs = tuple("ijklmnopqrstuvwxyzabcdefgh")
idxs = dummy_idxs + tuple("0")

latex_names = (
    ("G", r"\mathcal{G}"),
    ("Lambda", r"\Lambda"),
    ("Omega", r"\Omega"),
    ("omega", r"\omega"),
    ("delta", r"\delta"),
)
letter_init = (
    ("a", "symmetric-tail"),
    ("B", "symmetric"),
    ("F", "2-idx"),
    ("Q", "involution"),
    ("Lambda", "involution"),
    ("V", "1-idx"),
)
letter_weight = (
    ("W", 1),
    ("V", 1),
)

GG = IndexedLetterMonoid(latex_names=latex_names, letter_init=letter_init,
                         letter_weight=letter_weight, dummy_idxs=dummy_idxs,
                         extra_idxs=("0",))
QQi = QuadraticField(-1, 'I', latex_name='i')
I = QQi(I)

PP = LaurentPolynomialRing(QQi, [f"p_{i}" for i in dummy_idxs]
                           + ['psi', 'mu', 'p', 'm', 'pi', 'D', 'ell', 'tau']
                           + ['alpha', 'beta', 'gamma', 'eta', 'nu', 'd']
                           + ['C_010', 'C_120', 'C_110', 'C_111'])
```

```
PP.latex_variable_names()
PP._latex_names[PP._names.index('ell')] = r"\ell"

FF = GG.algebra(PP)

PP.inject_variables()

for letter in ["a", "Q", "F", "W", "V", "B", "f", "Omega", "delta"]:
    globals()[letter], = FF.get_constructors([letter])

def P(i): return PP.gens_dict()[f"p_{i}"]
def Qs(idxs=()): return FF(GG([("Q", (";",) + tuple(idxs))]))
def fs(idxs=()): return FF(GG([("f", (";",) + tuple(idxs))]))
G = FF(GG([("G", ())]))
Lambda = FF(GG([("Lambda", ())]))
```

For example:

$$\texttt{a("ijk")} * \texttt{G} * \texttt{Lambda} * \texttt{Lambda} * \texttt{a("ikj")} = a_{ijk}\mathcal{G}a_{ijk} \tag{1}$$

$$\texttt{a("ijk")} * \texttt{G} * \texttt{delta("ij")} * \texttt{delta("jk")} * \texttt{delta("ik")} = \delta_{ij}\delta_{ik}a_{iii}\mathcal{G}\,. \tag{2}$$

For the case where the indices are dummy indices that are all summed over, we should implement relabeling them. Also, in such convention $\delta$ can be dropped (after adjusting indices). So, to implement such operations:

**Code 3** (Relabeling, dummy sums)**.**

```
from indexed_letter_monoid import distributive_op, relabel as _relabel

def relabel(expr, idxs=dummy_idxs, keep=(), map=None):
    """Relabel dummy indices in *expr*"""
    return _relabel(expr, idxs=idxs, keep=keep, map=map,
                   cmap=lambda c, ix: c.subs({P(i): P(j) for i, j in ix.items()}))

def letters(expr):
    """Return all letters in the expression"""
    res = set()
    monomials = [expr] if expr.parent() is GG else expr.monomials()
    for m in monomials:
        res.update(v.letter for v in GG(m))
    return res

def idxset(m, c):
    """Return non-delta and delta indices and gradient order"""
    mc_ix = set()
    delta_ix = set()
    order = 0
    for letter, idx in m.value:
        if letter == "delta":
            delta_ix.add(idx)
        else:
            mc_ix.update(idx)
            order += len(idx)
    if c.parent() is PP:
        for exps, term in c.iterator_exp_coeff():
            mc_ix.update(idxs[k] for k, v in enumerate(exps[:len(dummy_idxs)]) if v != 0)
    return mc_ix, delta_ix, order

def idxset_expr(expr):
    idx = set()
```

```
        for m, c in expr:
            idx.update(idxset(m, c)[0])
        return idx

    @distributive_op
    def dummy_sum_delta(m, c, algebra, ndim=3):
        """Eliminate delta_ij by summing over dummy indices"""
        # Adjust prefactor indices; monomials do it themselves
        mc_ix, delta_ix, order = idxset(m, c)
        csub = {P(i1): P(i0) for i0, i1 in delta_ix if i1 in dummy_idxs}
        # Each free delta_ij produces factor of ndim under summation
        free_count = sum(i0 not in mc_ix and i1 not in mc_ix
                         and i0 in dummy_idxs and i1 in dummy_idxs
                         for i0, i1 in delta_ix)
        p = [v for v in m if v.letter != "delta"]
        return [(p, ndim**free_count * c.subs(csub))]

    def mul_relabel(a, b, idxs=dummy_idxs, keep=()):
        """Multiply expressions, relabeling duplicate indices"""
        a = relabel(a, keep=keep)
        free_idxs = set(idxs) - idxset_expr(a) - set(keep)
        return relabel(a * relabel(b, idxs=free_idxs, keep=keep), idxs=idxs, keep=keep)
```

For example,

$$\texttt{relabel}(\psi a_j a_i a_{ij} + p_j p_k a_k a_j a_{jk}) = (p_i p_j + \psi)\, a_i a_j a_{ji}\,, \tag{3}$$

$$\texttt{dummy\_sum\_delta}(p_i p_j \delta_{ij} \delta_{kl} \delta_{mm} a_{ii}) = 9 p_i^2 a_{ii}\,. \tag{4}$$

### B. Natural units

We will express lengths in units of $\ell := v_F \tau$, and energies in units of $1/\tau$. The results also depend on the dimensionless parameter $\psi = 2\mu\tau = p_F \ell$. We also note $\mu = \psi/(2\tau)$, $m = \tau\psi/\ell^2$.

```
subs_dimensionless = {tau: 1, ell: 1, m: psi, mu: psi/2}

@distributive_op
def reintroduce_units(m, c, algebra):
    ni = sum(ix in dummy_idxs for letter, idx in m.value for ix in idx)
    n0 = sum(ix == "0" for letter, idx in m.value for ix in idx)
    nOmega = sum(letter == "Omega" for letter, idx in m.value)
    return [(m, c * tau**(n0+nOmega) * ell**ni)]
```

### C. Momentum direction average

Average over $S^d \subset \mathbb{R}^{d+1}$ is

$$\int_{S^d} \frac{\mathrm{d}S_p}{V(S^d)} p_{i_1} \dots p_{i_n} = \frac{p^n (d-1)!!}{(n+d-1)!!} \sum_{C \in \text{pair combinations}} \prod_{(i_a, i_b) \in C} \delta_{i_a, i_b} \tag{5}$$

The double factorial is here defined as usual, with $0!! = 1$, $(-1)!! = 1$.

And so:

**Code 4** (Momentum direction average)**.**

```
def double_factorial(n):
    return Integer(prod(j for j in range(n, 0, -2)))

def pair_combinations(s):
    if not s:
        yield ()
    else:
        for k in range(1, len(s)):
            for c in pair_combinations(s[1:k] + s[k+1:]):
                yield ((s[0], s[k]),) + c

@distributive_op
def avg_p(m, c, algebra, ndim=3):
    """Average momenta over d-sphere."""
    res = []
    p = PP.gens_dict()['p']
    psub = {P(j): p for j in dummy_idxs}
    for c0, term in c:
        exps, = term.exponents()
        pexps = exps[:len(dummy_idxs)]
        if sum(pexps) % 2 != 0:
            continue  # odd in momenta -> 0
        ix = []
        for k, pexp in enumerate(pexps):
            ix += [dummy_idxs[k]]*pexp
        dim_fac = double_factorial(ndim - 2) / double_factorial(sum(pexps) + ndim - 2)
        c2 = dim_fac * c0 * term.subs(psub)
        for combs in pair_combinations(ix):
            m2 = m * GG(delta(comb) for comb in combs)
            res.append((m2, c2))
    return res

def avg_p_dummy_sum(expr, ndim=3):
    return relabel(dummy_sum_delta(avg_p(expr, ndim=ndim), ndim=ndim))
```

Example:

$$p_i p_j \mapsto \frac{1}{3} p^2 \delta_{ij} \tag{6}$$

$$p_i p_j p_k p_l \mapsto \frac{1}{15} p^4 \delta_{ij}\delta_{kl} + \frac{1}{15} p^4 \delta_{ik}\delta_{jl} + \frac{1}{15} p^4 \delta_{il}\delta_{jk} \tag{7}$$

$$p_i p_j^2 p_k^3 \mapsto \tfrac{4}{35} p^6 \delta_{ij}\delta_{ik} + \tfrac{1}{35} p^6 \delta_{ik}\delta_{jj} \tag{8}$$

Example (dummy summation assumed):

$$(p_i p_j + \mu)\, a_i a_j + 2 p_i p_j p_k a_i a_{jk} + p_i p_j p_k p_l \psi a_{ijk} a_l \mapsto \frac{1}{3} p^2 a_i a_i + \mu a_i a_j + \frac{2}{15} \psi p^4 a_{iij} a_j + \frac{1}{15} \psi p^4 a_{ijj} a_i \tag{9}$$

$$p_i^3 p_j p_k p_l a_i \mathcal{G} a_j a_k \mathcal{G} a_l \mapsto \frac{2}{35} p^6 a_i \mathcal{G} a_i a_i \mathcal{G} a_i + \frac{1}{35} p^6 a_i \mathcal{G} a_i a_j \mathcal{G} a_j + \frac{1}{35} p^6 a_i \mathcal{G} a_j a_i \mathcal{G} a_j + \frac{1}{35} p^6 a_i \mathcal{G} a_j a_j \mathcal{G} a_i \tag{10}$$

$$p_i p_j \mapsto p^2 \tag{11}$$

$$p_i p_j p_k p_l \mapsto \frac{9}{5} p^4 \tag{12}$$

$$p_i p_j^3 \mapsto \frac{3}{5} p^4 \tag{13}$$

1. Wigner convolution product

We also need the two-sided derivative operator and its powers,

$$A(\overleftrightarrow{D})^n B := A(\overleftarrow{\partial}_{R_i}\overrightarrow{\partial}_{p_i} - \overleftarrow{\partial}_{p_j}\overrightarrow{\partial}_{R_j})^n B = \sum_{k=0}^{n} \binom{n}{k} (-1)^{n-k} [\partial_{R_{i_1}} \cdots \partial_{R_{i_k}} \partial_{p_{j_1}} \cdots \partial_{p_{j_{n-k}}} A][\partial_{p_{i_1}} \cdots \partial_{p_{i_k}} \partial_{R_{j_1}} \cdots \partial_{R_{j_{n-k}}} B] \,. \tag{14}$$

For this, we define derivative operators (we'll consider extra indices on $a$ as plain derivatives, and, for later use, otherwise as covariant derivatives)

**Code 5** (Derivative operators)**.**

```
D_constant = ("Lambda", "G", "delta")
D_covariant = ("F", "Q", "W", "V", "f", "delta", "Omega")
D_plain = ("a", "B") + D_constant

@distributive_op
def _deriv_R(m, c, algebra, i, covariant=False, check=True):
    res = []
    if i not in idxs:
        raise DifferentiationError(f"Invalid diff. index {i}")
    for k, (letter, idx) in enumerate(m.value):
        _check_diff(letter, idx, covariant, check=check)
        if letter in D_constant: continue
        value = m.value[:k] + ((letter, idx + (i,)),) + m.value[k+1:]
        res.append((value, c))
    return res

def _check_diff(letter, idx, covariant, check=True):
    if not check:
        return
    # Sanity check we're not mixing up types of indices
    if ";" in idx:
        raise DifferentiationError(f"Cannot differentiate symmetrized")
    if not (covariant and letter in D_covariant or not covariant and letter in D_plain):
        raise DifferentiationError(f"Mixed plain/covariant derivatives: {letter!r} {covariant}")

class DifferentiationError(ValueError):
    pass

@distributive_op
def _deriv_p(m, c, algebra, i):
    res = []
    mm = PP.gens_dict()['m']
    assert i in idxs
    for j in dummy_idxs:
        res.append((m * GG(delta((j, i))), diff(c, P(j))))
    for k, (letter, idx) in enumerate(m.value):
        if letter == "G" and i in dummy_idxs:
            c2 = P(i) / mm * c
            value = m.value[:k] + (("G", ()), ("G", ())) + m.value[k+1:]
            res.append((value, c2))
    return res

def deriv_p(expr, idxs):
    for i in idxs:
        expr = _deriv_p(expr, i)
    return expr
```

```
def deriv_R(expr, idxs, covariant=False, check=True):
    for i in idxs:
        expr = _deriv_R(expr, i, covariant=covariant, check=check)
    return expr
```

For example,

$$\partial_{R_k}(a_{ii}\mathcal{G}) = a_{iik}\mathcal{G}\,, \tag{15}$$

$$\partial_{p_k}(p_i p_j a_{ij}\mathcal{G}) = \left(p_i p_j p_k m^{-1}\right) a_{ij}\mathcal{G}\mathcal{G} + p_j\delta_{ik}a_{ij}\mathcal{G} + p_i\delta_{jk}a_{ij}\mathcal{G}\,. \tag{16}$$

The two-sided derivative can then be built. We'll limit the order of terms to generate here. The order of a term is equal to the number of indices in its monomial (excluding $\delta$). It is assumed the indices are dummy indices summed over, and those on the left and right operands are independent, and so they will be relabeled.

**Code 6** (Two-sided derivative)**.**

```
def D_leftright(expr1, expr2, n=1, max_order=4, ndim=3):
    algebra = expr1.parent()
    ring = algebra.base_ring()
    res = algebra(0)
    for (m1, c1), (m2, c2) in cartesian_product_iterator([expr1, expr2]):
        # Find out indices on the left and the right
        mc_idx1, d_idx1, order_1 = idxset(m1, c1)
        mc_idx2, d_idx2, order_2 = idxset(m2, c2)
        idx1 = (mc_idx1 | d_idx1) & set(dummy_idxs)
        idx2 = (mc_idx2 | d_idx2) & set(dummy_idxs)

        if order_1 + order_2 + n > max_order:
            continue
        if len(idx1) + len(idx2) + n > len(dummy_idxs):
            raise ValueError("ran out of indices!")

        # Relabel indices
        new_idx1 = dummy_idxs[:len(idx1)]
        new_idx2 = dummy_idxs[len(idx1):len(idx1)+len(idx2)]
        A = relabel(algebra.term(m1, c1), new_idx1)
        B = relabel(algebra.term(m2, c2), new_idx2)

        # D^n with new dummy indices
        dummy = dummy_idxs[len(idx1)+len(idx2):len(idx1)+len(idx2)+n]
        for k in range(n + 1):
            coef = (-1)**(n-k) * binomial(n, k)
            res += dummy_sum_delta(coef * deriv_p(deriv_R(A, dummy[:k]), dummy[k:])
                                   * deriv_R(deriv_p(B, dummy[:k]), dummy[k:]), ndim=ndim)
    return relabel(res)
```

For example, (NB: up to order 4!)

$$(a_{ii}\mathcal{G})(\overleftrightarrow{D})^0(a_{ii}\mathcal{G}) = a_{ii}\mathcal{G}a_{jj}\mathcal{G}\,, \tag{17}$$

$$(a_{ii}\mathcal{G})\overleftrightarrow{D}(a_{ii}\mathcal{G}) = 0\,, \tag{18}$$

$$(p_i a_i\mathcal{G})\overleftrightarrow{D}(p_i a_i\mathcal{G}) = (-p_j)\, a_i\mathcal{G}a_{ji}\mathcal{G} + p_i a_{ij}\mathcal{G}a_j\mathcal{G} + \left(-p_i p_j p_k m^{-1}\right) a_i\mathcal{G}\mathcal{G}a_{jk}\mathcal{G} + \left(p_i p_j p_k m^{-1}\right) a_{ij}\mathcal{G}a_k\mathcal{G}\mathcal{G}\,. \tag{19}$$

The product $A \otimes B = \sum_{n=0}^{\infty} \frac{i^n}{2^n n!} A(\overleftrightarrow{D})^n B$ truncated to a fixed order then is:

**Code 7** (Convolution product).

```
def W_product(A, B, max_order=4, ndim=3):
    res = 0
    for n in range(max_order + 2):
        term = D_leftright(A, B, n, max_order, ndim=ndim) * ((I/2)**n / factorial(n))
        res += term
    return res
```

For example (again, truncation after order 4),

$$\begin{aligned}\mathcal{G} \otimes a_i a_i = {} & \mathcal{G} a_i a_i + \left(\left(-\tfrac{1}{2} i\right) p_j m^{-1}\right) \mathcal{G}\mathcal{G} a_i a_{ij} + \left(\left(-\tfrac{1}{2} i\right) p_j m^{-1}\right) \mathcal{G}\mathcal{G} a_{ij} a_i + \left(\left(-\tfrac{1}{4}\right) m^{-1}\right) \mathcal{G}\mathcal{G} a_{ij} a_{ij} + \\ & \left(\left(-\tfrac{1}{8}\right) m^{-1}\right) \mathcal{G}\mathcal{G} a_i a_{ijj} + \left(\left(-\tfrac{1}{8}\right) m^{-1}\right) \mathcal{G}\mathcal{G} a_{ijj} a_i + \left(\left(-\tfrac{1}{2}\right) p_j p_k m^{-2}\right) \mathcal{G}\mathcal{G}\mathcal{G} a_{ij} a_{ik} + \\ & \left(\left(-\tfrac{1}{4}\right) p_j p_k m^{-2}\right) \mathcal{G}\mathcal{G}\mathcal{G} a_i a_{ijk} + \left(\left(-\tfrac{1}{4}\right) p_j p_k m^{-2}\right) \mathcal{G}\mathcal{G}\mathcal{G} a_{ijk} a_i \,,\end{aligned} \tag{20}$$

$$\begin{aligned}\langle \mathcal{G} \otimes a_i a_i \rangle = {} & \mathcal{G} a_i a_i + \left(\left(-\tfrac{1}{4}\right) m^{-1}\right) \mathcal{G}\mathcal{G} a_{ij} a_{ij} + \left(\left(-\tfrac{1}{8}\right) m^{-1}\right) \mathcal{G}\mathcal{G} a_i a_{ijj} + \left(\left(-\tfrac{1}{8}\right) m^{-1}\right) \mathcal{G}\mathcal{G} a_{ijj} a_i + \\ & \left(\left(-\tfrac{1}{6}\right) p^2 m^{-2}\right) \mathcal{G}\mathcal{G}\mathcal{G} a_{ij} a_{ij} + \left(\left(-\tfrac{1}{12}\right) p^2 m^{-2}\right) \mathcal{G}\mathcal{G}\mathcal{G} a_i a_{ijj} + \\ & \left(\left(-\tfrac{1}{12}\right) p^2 m^{-2}\right) \mathcal{G}\mathcal{G}\mathcal{G} a_{ijj} a_i \,,\end{aligned} \tag{21}$$

and truncated to order 6 (again, indices on left and right are considered distinct dummy indices):

$$\begin{aligned}\mathcal{G} a_i a_i \otimes \mathcal{G} a_{ii} = {} & \mathcal{G} a_i a_i \mathcal{G} a_{jj} + \left(\left(\tfrac{1}{2} i\right) p_j m^{-1}\right) \mathcal{G} a_i a_{ij} \mathcal{G}\mathcal{G} a_{kk} + \left(\left(\tfrac{1}{2} i\right) p_j m^{-1}\right) \mathcal{G} a_{ij} a_i \mathcal{G}\mathcal{G} a_{kk} + \\ & \left(\left(-\tfrac{1}{4}\right) m^{-1}\right) \mathcal{G} a_{ij} a_{ij} \mathcal{G}\mathcal{G} a_{kk} + \left(\left(-\tfrac{1}{2} i\right) p_k m^{-1}\right) \mathcal{G}\mathcal{G} a_i a_i \mathcal{G} a_{jjk} + \\ & \left(\left(-\tfrac{1}{8}\right) m^{-1}\right) \mathcal{G} a_i a_{ijj} \mathcal{G}\mathcal{G} a_{kk} + \left(\left(-\tfrac{1}{8}\right) m^{-1}\right) \mathcal{G} a_{ijj} a_i \mathcal{G}\mathcal{G} a_{kk} + \\ & \left(\left(-\tfrac{1}{8}\right) m^{-1}\right) \mathcal{G}\mathcal{G} a_i a_i \mathcal{G} a_{jjkk} + \left(\left(-\tfrac{1}{2}\right) p_j p_k m^{-2}\right) \mathcal{G} a_{ij} a_{ik} \mathcal{G}\mathcal{G}\mathcal{G} a_{ll} + \\ & \left(\tfrac{1}{4} p_j p_l m^{-2}\right) \mathcal{G}\mathcal{G} a_i a_{ij} \mathcal{G}\mathcal{G} a_{kkl} + \left(\tfrac{1}{4} p_j p_l m^{-2}\right) \mathcal{G}\mathcal{G} a_{ij} a_i \mathcal{G}\mathcal{G} a_{kkl} + \\ & \left(\left(-\tfrac{1}{4}\right) p_j p_k m^{-2}\right) \mathcal{G} a_i a_{ijk} \mathcal{G}\mathcal{G}\mathcal{G} a_{ll} + \left(\left(-\tfrac{1}{4}\right) p_j p_k m^{-2}\right) \mathcal{G} a_{ijk} a_i \mathcal{G}\mathcal{G}\mathcal{G} a_{ll} + \\ & \left(\left(-\tfrac{1}{4}\right) p_k p_l m^{-2}\right) \mathcal{G}\mathcal{G}\mathcal{G} a_i a_i \mathcal{G} a_{jjkl} \,,\end{aligned} \tag{22}$$

$$\begin{aligned}\langle \mathcal{G} a_i a_i \otimes \mathcal{G} a_{ii} \rangle = {} & \mathcal{G} a_i a_i \mathcal{G} a_{jj} + \left(\left(-\tfrac{1}{4}\right) m^{-1}\right) \mathcal{G} a_{ij} a_{ij} \mathcal{G}\mathcal{G} a_{kk} + \left(\left(-\tfrac{1}{8}\right) m^{-1}\right) \mathcal{G} a_i a_{ijj} \mathcal{G}\mathcal{G} a_{kk} + \\ & \left(\left(-\tfrac{1}{8}\right) m^{-1}\right) \mathcal{G} a_{ijj} a_i \mathcal{G}\mathcal{G} a_{kk} + \left(\left(-\tfrac{1}{8}\right) m^{-1}\right) \mathcal{G}\mathcal{G} a_i a_i \mathcal{G} a_{jjkk} + \\ & \left(\left(-\tfrac{1}{6}\right) p^2 m^{-2}\right) \mathcal{G} a_{ij} a_{ij} \mathcal{G}\mathcal{G}\mathcal{G} a_{kk} + \left(\tfrac{1}{12} p^2 m^{-2}\right) \mathcal{G}\mathcal{G} a_i a_{ij} \mathcal{G}\mathcal{G} a_{kjk} + \\ & \left(\tfrac{1}{12} p^2 m^{-2}\right) \mathcal{G}\mathcal{G} a_{ij} a_i \mathcal{G}\mathcal{G} a_{kjk} + \left(\left(-\tfrac{1}{12}\right) p^2 m^{-2}\right) \mathcal{G} a_i a_{ijj} \mathcal{G}\mathcal{G}\mathcal{G} a_{kk} + \\ & \left(\left(-\tfrac{1}{12}\right) p^2 m^{-2}\right) \mathcal{G} a_{ijj} a_i \mathcal{G}\mathcal{G}\mathcal{G} a_{kk} + \left(\left(-\tfrac{1}{12}\right) p^2 m^{-2}\right) \mathcal{G}\mathcal{G}\mathcal{G} a_i a_i \mathcal{G} a_{jjkk} \,,\end{aligned} \tag{23}$$

### D. Momentum integration and $p_F \ell$ expansion

We also need to implement the momentum integration from the previous subsections,

**Code 8** (Momentum integration).

```
@distributive_op
def integrate_p(m, c, algebra, ndim=3, order=-1):
    """Compute I/(pi*nu_F)*sum_p expr(p)"""
    p = PP.gens_dict()['p']
    mm = PP.gens_dict()['m']
    N = sum(letter == "G" for letter, idx in m.value)
    res = []
    for coef, term in c:
        deg_p = term.degree(p)
        assert deg_p % 2 == 0
        beta = deg_p // 2
        c_0 = coef * term.subs({p: 1})
```

```
        for alphas in cartesian_product_iterator([[0,1]]*N):
            n = sum(alphas)
            C, is_convergent = C_tilde(beta, N, n, order=order, ndim=ndim, regularize=False)
            C = ((2*mm)**beta * mu**(beta + 1 - N)
                 * PP(C.subs({SR.pi(): PP.gens_dict()['pi']})))
            ait = iter(alphas)
            value = []
            for letter, idx in m.value:
                if letter == "G":
                    if next(ait):
                        letter = "Lambda"
                    else:
                        continue
                value.append((letter, idx))

            res.append((value, c_0 * C))
    return res
```

For example, with error $\mathcal{O}(\psi^{-1})$,

$$\fint \mathrm{d}p \left\langle \left(\frac{1}{2}i\right) p_i p_k \mathcal{G}\mathcal{G} a_i + \left(\left(-i\right) p_i p_k\right) \mathcal{G} a_i \mathcal{G} + \left(\frac{1}{2}i\right) p_i p_k a_i \mathcal{G}\mathcal{G} \right\rangle = \tfrac{1}{3}\psi m \delta_{ik} a_i + \left(\left(-\tfrac{1}{3}\right)\psi m\right) \delta_{ik} \Lambda a_i \Lambda \tag{24}$$

$$\fint \mathrm{d}p \left\langle \mathcal{G} a_i a_i + p_i p_k \mathcal{G} a_i a_k \right\rangle = C_{010} a_i a_i + \Lambda a_i a_i + \tfrac{2}{3}\mu m C_{110} \delta_{ik} a_i a_i + \tfrac{2}{3}\mu m C_{111} \delta_{ik} \Lambda a_i a_i \quad . \tag{25}$$

We represent divergent integrals in terms of the constants $C_{\beta N n}$.

## E. Tr ln expansion

The main object of our exercise, the ln gradient expansion, can now be done. We don't include terms with $a_0$ here yet: that discussion is postponed to Sec. III.J. We will also now switch to the dimensionless units in Sec. III.B:

**Code 9** (Gradient expansion)**.**

```
def log_one_plus_expansion(X, max_order=4, limit=100, ndim=3):
    res = Y = X
    for n in range(1, limit):
        Y = W_product(Y, X, max_order=max_order, ndim=ndim)
        if Y == 0:
            break
        res += (-1)**n / (n+1) * Y
    return res

def gradient_expansion(max_order, ndim=3, reverse=False, igorder=-1, with_a0=False,
                       with_ai=True):
    Z = FF(0)
    if with_ai:
        Z += 1/(2*m)*(2*P('i')*a('i') - a('i')*a('i'))
    if with_a0:
        Z += a("0")
    if not reverse:
        X = W_product(Z, G, max_order=max_order, ndim=ndim)
    else:
        X = W_product(G, Z, max_order=max_order, ndim=ndim)
```

```
        log = log_one_plus_expansion(X, max_order=max_order, ndim=ndim)
        avg_log = integrate_p(avg_p_dummy_sum(log, ndim=ndim), ndim=ndim, order=igorder)
        return (X, log, avg_log.map_coefficients(lambda z: z.subs(subs_dimensionless)))

    X_2, log_2, avg_log_2_a = gradient_expansion(max_order=2)
```

$$\mathtt{X\_2} = \left(p_i m^{-1}\right) a_i \mathcal{G} + \left(\left(-\frac{1}{2}\right) m^{-1}\right) a_i a_i \mathcal{G} + \left(\left(\frac{1}{2} i\right) p_i p_j m^{-2}\right) a_{ij} \mathcal{G}\mathcal{G}\,, \tag{26}$$

$$\mathtt{log\_2} = \left(p_i m^{-1}\right) a_i \mathcal{G} + \left(\left(-\frac{1}{2}\right) m^{-1}\right) a_i a_i \mathcal{G} + \left(\left(\frac{1}{2} i\right) p_i p_j m^{-2}\right) a_{ij} \mathcal{G}\mathcal{G} + \left(\left(-\frac{1}{2}\right) p_i p_j m^{-2}\right) a_i \mathcal{G} a_j \mathcal{G}\,, \tag{27}$$

$$\mathtt{avg\_log\_2} = \left(\tfrac{1}{6} + \left(\tfrac{1}{3} i\right) \psi^{-1} C_{120}\right) a_{ii} + \left(\left(-\tfrac{1}{2}\right) \psi^{-1} C_{010} + \left(-\tfrac{1}{3}\right) \psi^{-1} C_{120}\right) a_i a_i + \tfrac{1}{6} i a_i \Lambda a_i \Lambda\,, \tag{28}$$

here to second order. Some of the terms are divergent. The divergent parts can be cancelled by subtracting a total spatial derivative $\partial_j(\frac{i p_i p_j}{2m} a_i \mathcal{G}^2)$ and a total momentum derivative $-\frac{1}{2m}\partial_{p_i}(p_j a_i a_j \mathcal{G}) = -\frac{p_i p_j}{2m^2} a_i a_j \mathcal{G}^2 - \frac{1}{2m} a_i a_i \mathcal{G}$ before integration. In the following, we will assume this was done,

```
    avg_log_2 = avg_log_2_a.map_coefficients(lambda z: z.subs({C_120: -3/2*C_010 - PP(C_tilde(1,2,2)[0])}))
```

which corresponds to an equivalent sum rule between the infinite constants.

Order 4 expansion comes out in the same way,

```
    X_4, log_4, avg_log_4 = gradient_expansion(max_order=4)
    avg_log_4 = avg_log_4 - avg_log_2_a
```

It has 106 terms.

All the fourth-order gradient terms have convergent prefactors. Hence, there's no need to subtract total momentum derivatives or regularize integrals in the fourth order.

$$\begin{aligned}
\mathtt{X_4} = {} & \left(p_i m^{-1}\right) a_i \mathcal{G} + \left(\left(-\tfrac{1}{2}\right) m^{-1}\right) a_i a_i \mathcal{G} + \left(\left(\tfrac{1}{2} i\right) p_i p_j m^{-2}\right) a_{ij} \mathcal{G}\mathcal{G} + \left(\left(-\tfrac{1}{8}\right) p_i m^{-2}\right) a_{ijj} \mathcal{G}\mathcal{G} + \left(\left(-\tfrac{1}{4} i\right) p_j m^{-2}\right) a_i a_{ij} \mathcal{G}\mathcal{G} + \left(\left(-\tfrac{1}{4} i\right) p_j m^{-2}\right) a_{ij} a_i \mathcal{G}\mathcal{G} + \\
& \left(\tfrac{1}{8} m^{-2}\right) a_{ij} a_{ij} \mathcal{G}\mathcal{G} + \left(\left(-\tfrac{1}{4}\right) p_i p_j p_k m^{-3}\right) a_{ijk} \mathcal{G}\mathcal{G}\mathcal{G} + \left(\tfrac{1}{16} m^{-2}\right) a_i a_{ijj} \mathcal{G}\mathcal{G} + \left(\tfrac{1}{16} m^{-2}\right) a_{ijj} a_i \mathcal{G}\mathcal{G} + \left(\left(-\tfrac{1}{12} i\right) p_i p_k m^{-3}\right) a_{ijjk} \mathcal{G}\mathcal{G}\mathcal{G} + \\
& \left(\left(-\tfrac{1}{24} i\right) p_i p_j m^{-3}\right) a_{ijkk} \mathcal{G}\mathcal{G}\mathcal{G} + \left(\tfrac{1}{4} p_j p_k m^{-3}\right) a_{ij} a_{ik} \mathcal{G}\mathcal{G}\mathcal{G} + \left(\tfrac{1}{8} p_j p_k m^{-3}\right) a_i a_{ijk} \mathcal{G}\mathcal{G}\mathcal{G} + \left(\tfrac{1}{8} p_j p_k m^{-3}\right) a_{ijk} a_i \mathcal{G}\mathcal{G}\mathcal{G} + \left(\left(-\tfrac{1}{8} i\right) p_i p_j p_k p_l m^{-4}\right) a_{ijkl} \mathcal{G}\mathcal{G}\mathcal{G}\mathcal{G}
\end{aligned}$$

$$\begin{aligned}
\mathtt{log_4} = {} & \left(p_i m^{-1}\right) a_i \mathcal{G} + \left(\left(-\tfrac{1}{2}\right) m^{-1}\right) a_i a_i \mathcal{G} + \left(\left(\tfrac{1}{2} i\right) p_i p_j m^{-2}\right) a_{ij} \mathcal{G}\mathcal{G} + \left(\left(-\tfrac{1}{8}\right) p_i m^{-2}\right) a_{ijj} \mathcal{G}\mathcal{G} + \left(\left(-\tfrac{1}{2}\right) p_i p_j m^{-2}\right) a_i \mathcal{G} a_j \mathcal{G} + \left(\left(\tfrac{1}{4} i\right) p_j m^{-2}\right) a_i \mathcal{G} a_{ji} \mathcal{G} + \\
& \left(\left(-\tfrac{1}{4} i\right) p_j m^{-2}\right) a_i a_{ij} \mathcal{G}\mathcal{G} + \left(\left(-\tfrac{1}{4} i\right) p_i m^{-2}\right) a_{ij} \mathcal{G} a_j \mathcal{G} + \left(\left(-\tfrac{1}{4} i\right) p_j m^{-2}\right) a_{ij} a_i \mathcal{G}\mathcal{G} + \left(\left(-\tfrac{1}{8}\right) m^{-2}\right) a_{ij} \mathcal{G} a_{ji} \mathcal{G} + \left(\tfrac{1}{8} m^{-2}\right) a_{ij} a_{ij} \mathcal{G}\mathcal{G} + \\
& \left(\left(-\tfrac{1}{4}\right) p_i p_j p_k m^{-3}\right) a_{ijk} \mathcal{G}\mathcal{G}\mathcal{G} + \left(\tfrac{1}{16} m^{-2}\right) a_i a_{ijj} \mathcal{G}\mathcal{G} + \left(\tfrac{1}{16} m^{-2}\right) a_{ijj} a_i \mathcal{G}\mathcal{G} + \left(\left(-\tfrac{1}{12} i\right) p_i p_k m^{-3}\right) a_{ijjk} \mathcal{G}\mathcal{G}\mathcal{G} + \left(\left(-\tfrac{1}{24} i\right) p_i p_j m^{-3}\right) a_{ijkk} \mathcal{G}\mathcal{G}\mathcal{G} + \\
& \left(\tfrac{1}{4} p_i m^{-2}\right) a_i \mathcal{G} a_j a_j \mathcal{G} + \left(\tfrac{1}{4} p_j m^{-2}\right) a_i a_i \mathcal{G} a_j \mathcal{G} + \left(\left(\tfrac{1}{4} i\right) p_i p_j p_k m^{-3}\right) a_i \mathcal{G}\mathcal{G} a_{jk} \mathcal{G} + \left(\left(-\tfrac{1}{4} i\right) p_i p_j p_k m^{-3}\right) a_i \mathcal{G} a_{jk} \mathcal{G}\mathcal{G} + \left(\left(-\tfrac{1}{4} i\right) p_i p_j p_k m^{-3}\right) a_{ij} \mathcal{G}\mathcal{G} a_k \mathcal{G} + \\
& \left(\left(-\tfrac{1}{4} i\right) p_i p_j p_k m^{-3}\right) a_{ij} \mathcal{G} a_k \mathcal{G}\mathcal{G} + \left(\left(-\tfrac{1}{8} i\right) m^{-2}\right) a_i \mathcal{G} a_j a_{ji} \mathcal{G} + \left(\left(-\tfrac{1}{8} i\right) m^{-2}\right) a_i \mathcal{G} a_{ji} a_j \mathcal{G} + \left(\left(\tfrac{1}{8} i\right) m^{-2}\right) a_i a_{ij} \mathcal{G} a_j \mathcal{G} + \left(\left(-\tfrac{1}{8}\right) p_i p_k m^{-3}\right) a_{ij} \mathcal{G}\mathcal{G} a_{jk} \mathcal{G} + \\
& \left(\left(-\tfrac{1}{8}\right) p_j p_k m^{-3}\right) a_{ij} \mathcal{G}\mathcal{G} a_{ki} \mathcal{G} + \left(\left(-\tfrac{1}{8}\right) p_i p_k m^{-3}\right) a_{ij} \mathcal{G}\mathcal{G} a_{kj} \mathcal{G} + \left(\tfrac{1}{8} p_i p_k m^{-3}\right) a_{ij} \mathcal{G} a_{jk} \mathcal{G}\mathcal{G} + \left(\left(-\tfrac{1}{8}\right) p_j p_k m^{-3}\right) a_{ij} \mathcal{G} a_{ki} \mathcal{G}\mathcal{G} + \\
& \left(\tfrac{1}{8} p_i p_k m^{-3}\right) a_{ij} \mathcal{G} a_{kj} \mathcal{G}\mathcal{G} + \left(\left(\tfrac{1}{8} i\right) m^{-2}\right) a_{ij} a_i \mathcal{G} a_j \mathcal{G} + \left(\tfrac{1}{4} p_j p_k m^{-3}\right) a_{ij} a_{ik} \mathcal{G}\mathcal{G}\mathcal{G} + \left(\tfrac{1}{8} p_j p_k m^{-3}\right) a_i \mathcal{G}\mathcal{G} a_{jik} \mathcal{G} + \left(\left(-\tfrac{1}{8}\right) p_j p_k m^{-3}\right) a_i \mathcal{G} a_{jik} \mathcal{G}\mathcal{G} + \\
& \left(\tfrac{1}{8} p_j p_k m^{-3}\right) a_i a_{ijk} \mathcal{G}\mathcal{G}\mathcal{G} + \left(\tfrac{1}{8} p_i p_j m^{-3}\right) a_{ijk} \mathcal{G}\mathcal{G} a_k \mathcal{G} + \left(\tfrac{1}{8} p_i p_k m^{-3}\right) a_{ijk} \mathcal{G} a_j \mathcal{G}\mathcal{G} + \left(\tfrac{1}{8} p_j p_k m^{-3}\right) a_{ijk} a_i \mathcal{G}\mathcal{G}\mathcal{G} + \left(\tfrac{1}{16} p_i p_j m^{-3}\right) a_i \mathcal{G}\mathcal{G} a_{jkk} \mathcal{G} + \\
& \left(\tfrac{1}{16} p_i p_j m^{-3}\right) a_i \mathcal{G} a_{jkk} \mathcal{G}\mathcal{G} + \left(\tfrac{1}{16} p_i p_k m^{-3}\right) a_{ijj} \mathcal{G}\mathcal{G} a_k \mathcal{G} + \left(\tfrac{1}{16} p_i p_k m^{-3}\right) a_{ijj} \mathcal{G} a_k \mathcal{G}\mathcal{G} + \left(\left(-\tfrac{1}{8} i\right) p_i p_j p_k p_l m^{-4}\right) a_{ijkl} \mathcal{G}\mathcal{G}\mathcal{G}\mathcal{G} + \\
& \left(\tfrac{1}{3} p_i p_j p_k m^{-3}\right) a_i \mathcal{G} a_j \mathcal{G} a_k \mathcal{G} + \left(\left(-\tfrac{1}{8}\right) m^{-2}\right) a_i a_i \mathcal{G} a_j a_j \mathcal{G} + \left(\left(-\tfrac{1}{8} i\right) p_i p_k m^{-3}\right) a_i \mathcal{G}\mathcal{G} a_j a_{jk} \mathcal{G} + \left(\left(-\tfrac{1}{8} i\right) p_i p_k m^{-3}\right) a_i \mathcal{G}\mathcal{G} a_{jk} a_j \mathcal{G} + \\
& \left(\left(-\tfrac{1}{6} i\right) p_j p_k m^{-3}\right) a_i \mathcal{G} a_j \mathcal{G} a_{ki} \mathcal{G} + \left(\left(-\tfrac{1}{6} i\right) p_i p_k m^{-3}\right) a_i \mathcal{G} a_j \mathcal{G} a_{kj} \mathcal{G} + \left(\left(\tfrac{1}{8} i\right) p_i p_k m^{-3}\right) a_i \mathcal{G} a_j a_{jk} \mathcal{G}\mathcal{G} + \left(\left(-\tfrac{1}{6} i\right) p_j p_k m^{-3}\right) a_i \mathcal{G} a_{ji} \mathcal{G} a_k \mathcal{G} + \\
& \left(\left(\tfrac{1}{6} i\right) p_i p_j m^{-3}\right) a_i \mathcal{G} a_{jk} \mathcal{G} a_k \mathcal{G} + \left(\left(\tfrac{1}{8} i\right) p_i p_k m^{-3}\right) a_i \mathcal{G} a_{jk} a_j \mathcal{G}\mathcal{G} + \left(\left(-\tfrac{1}{8} i\right) p_j p_k m^{-3}\right) a_i a_i \mathcal{G}\mathcal{G} a_{jk} \mathcal{G} + \left(\left(\tfrac{1}{8} i\right) p_j p_k m^{-3}\right) a_i a_i \mathcal{G} a_{jk} \mathcal{G}\mathcal{G} + \\
& \left(\left(\tfrac{1}{8} i\right) p_j p_k m^{-3}\right) a_i a_{ij} \mathcal{G}\mathcal{G} a_k \mathcal{G} + \left(\left(\tfrac{1}{8} i\right) p_j p_k m^{-3}\right) a_i a_{ij} \mathcal{G} a_k \mathcal{G}\mathcal{G} + \left(\left(-\tfrac{1}{4}\right) p_i p_j p_k p_l m^{-4}\right) a_{ij} \mathcal{G}\mathcal{G}\mathcal{G} a_{kl} \mathcal{G} + \left(\left(\tfrac{1}{8} i\right) p_i p_j m^{-3}\right) a_{ij} \mathcal{G}\mathcal{G} a_k a_k \mathcal{G} + \\
& \left(\left(\tfrac{1}{6} i\right) p_i p_k m^{-3}\right) a_{ij} \mathcal{G} a_j \mathcal{G} a_k \mathcal{G} + \left(\left(\tfrac{1}{6} i\right) p_i p_k m^{-3}\right) a_{ij} \mathcal{G} a_k \mathcal{G} a_j \mathcal{G} + \left(\left(\tfrac{1}{8} i\right) p_i p_j m^{-3}\right) a_{ij} \mathcal{G} a_k a_k \mathcal{G}\mathcal{G} + \left(\tfrac{1}{4} p_i p_j p_k p_l m^{-4}\right) a_{ij} \mathcal{G} a_{kl} \mathcal{G}\mathcal{G}\mathcal{G} + \\
& \left(\left(\tfrac{1}{8} i\right) p_j p_k m^{-3}\right) a_{ij} a_i \mathcal{G}\mathcal{G} a_k \mathcal{G} + \left(\left(\tfrac{1}{8} i\right) p_j p_k m^{-3}\right) a_{ij} a_i \mathcal{G} a_k \mathcal{G}\mathcal{G} + \left(\tfrac{1}{8} p_i p_j p_k p_l m^{-4}\right) a_i \mathcal{G}\mathcal{G}\mathcal{G} a_{jkl} \mathcal{G} + \left(\left(-\tfrac{1}{8}\right) p_i p_j p_k p_l m^{-4}\right) a_i \mathcal{G}\mathcal{G} a_{jkl} \mathcal{G}\mathcal{G} + \\
& \left(\tfrac{1}{8} p_i p_j p_k p_l m^{-4}\right) a_i \mathcal{G} a_{jkl} \mathcal{G}\mathcal{G}\mathcal{G} + \left(\tfrac{1}{8} p_i p_j p_k p_l m^{-4}\right) a_{ijk} \mathcal{G}\mathcal{G}\mathcal{G} a_l \mathcal{G} + \left(\tfrac{1}{8} p_i p_j p_k p_l m^{-4}\right) a_{ijk} \mathcal{G}\mathcal{G} a_l \mathcal{G}\mathcal{G} + \left(\tfrac{1}{8} p_i p_j p_k p_l m^{-4}\right) a_{ijk} \mathcal{G} a_l \mathcal{G}\mathcal{G}\mathcal{G} + \\
& \left(\left(-\tfrac{1}{6}\right) p_i p_j m^{-3}\right) a_i \mathcal{G} a_j \mathcal{G} a_k a_k \mathcal{G} + \left(\left(-\tfrac{1}{6}\right) p_i p_k m^{-3}\right) a_i \mathcal{G} a_j a_j \mathcal{G} a_k \mathcal{G} + \left(\left(-\tfrac{1}{6}\right) p_j p_k m^{-3}\right) a_i a_i \mathcal{G} a_j \mathcal{G} a_k \mathcal{G} + \left(\left(-\tfrac{1}{6} i\right) p_i p_j p_k p_l m^{-4}\right) a_i \mathcal{G}\mathcal{G} a_j \mathcal{G} a_{kl} \mathcal{G} + \\
& \left(\left(-\tfrac{1}{6} i\right) p_i p_j p_k p_l m^{-4}\right) a_i \mathcal{G}\mathcal{G} a_{jk} \mathcal{G} a_l \mathcal{G} + \left(\left(-\tfrac{1}{6} i\right) p_i p_j p_k p_l m^{-4}\right) a_i \mathcal{G} a_j \mathcal{G}\mathcal{G} a_{kl} \mathcal{G} + \left(\left(\tfrac{1}{6} i\right) p_i p_j p_k p_l m^{-4}\right) a_i \mathcal{G} a_j \mathcal{G} a_{kl} \mathcal{G}\mathcal{G} + \\
& \left(\left(\tfrac{1}{6} i\right) p_i p_j p_k p_l m^{-4}\right) a_i \mathcal{G} a_{jk} \mathcal{G}\mathcal{G} a_l \mathcal{G} + \left(\left(\tfrac{1}{6} i\right) p_i p_j p_k p_l m^{-4}\right) a_i \mathcal{G} a_{jk} \mathcal{G} a_l \mathcal{G}\mathcal{G} + \left(\left(\tfrac{1}{6} i\right) p_i p_j p_k p_l m^{-4}\right) a_{ij} \mathcal{G}\mathcal{G} a_k \mathcal{G} a_l \mathcal{G} + \\
& \left(\left(\tfrac{1}{6} i\right) p_i p_j p_k p_l m^{-4}\right) a_{ij} \mathcal{G} a_k \mathcal{G}\mathcal{G} a_l \mathcal{G} + \left(\left(\tfrac{1}{6} i\right) p_i p_j p_k p_l m^{-4}\right) a_{ij} \mathcal{G} a_k \mathcal{G} a_l \mathcal{G}\mathcal{G} + \left(\left(-\tfrac{1}{4}\right) p_i p_j p_k p_l m^{-4}\right) a_i \mathcal{G} a_j \mathcal{G} a_k \mathcal{G} a_l \mathcal{G}
\end{aligned}$$

$$\begin{aligned}
\mathtt{avg_log_4} = {} & \left(-\tfrac{1}{30} i + \left(-\tfrac{1}{16} i\right) \psi^{-2}\right) a_i a_{ijj} + \left(-\tfrac{1}{15} i\right) a_i a_{jij} + \left(\left(-\tfrac{1}{12}\right) \psi^{-2}\right) a_i a_j a_{ij} + \left(\tfrac{1}{24} \psi^{-2}\right) a_i a_j a_{ji} + \left(\tfrac{1}{12} \psi^{-2}\right) a_i a_{ij} a_j + \left(\left(-\tfrac{1}{24}\right) \psi^{-2}\right) a_i a_{ji} a_j + \\
& \left(\tfrac{1}{24} \psi^{-2}\right) a_i a_i a_{jj} + \left(\left(-\tfrac{1}{24}\right) \psi^{-2}\right) a_i a_{jj} a_i + \left(\tfrac{1}{12} \psi^{-1}\right) a_{ii} \Lambda a_{jj} + \left(\left(-\tfrac{1}{12}\right) \psi^{-1}\right) a_{ii} a_{jj} \Lambda + \left(\tfrac{1}{12} \psi^{-1}\right) a_i \Lambda a_{jij} + \left(\left(-\tfrac{1}{12}\right) \psi^{-1}\right) a_i a_{jij} \Lambda + \\
& \left(-\tfrac{1}{120} i + \left(\tfrac{3}{64} i\right) \psi^{-2}\right) a_i a_i a_j a_j + \left(-\tfrac{1}{120} i + \left(-\tfrac{5}{64} i\right) \psi^{-2}\right) a_i a_j a_i a_j + \left(-\tfrac{1}{120} i + \left(\tfrac{3}{64} i\right) \psi^{-2}\right) a_i a_j a_j a_i + \left(\left(-\tfrac{1}{12} i\right) \psi^{-1}\right) a_i \Lambda a_j a_{ji} + \\
& \left(\left(\tfrac{1}{18} i\right) \psi^{-1}\right) a_i \Lambda a_{ij} a_j + \left(\left(-\tfrac{1}{12} i\right) \psi^{-1}\right) a_i \Lambda a_{ji} a_j + \left(\left(-\tfrac{1}{18} i\right) \psi^{-1}\right) a_i a_j a_{ij} \Lambda + \left(\left(\tfrac{1}{36} i\right) \psi^{-1}\right) a_i a_j a_{ji} \Lambda + \left(\left(-\tfrac{1}{18} i\right) \psi^{-1}\right) a_i a_{ji} \Lambda a_j + \\
& \left(\left(\tfrac{1}{36} i\right) \psi^{-1}\right) a_i a_{ji} a_j \Lambda + \left(\left(\tfrac{1}{36} i\right) \psi^{-1}\right) a_i \Lambda a_i a_{jj} + \left(\left(\tfrac{1}{36} i\right) \psi^{-1}\right) a_i \Lambda a_{jj} a_i + \left(\left(-\tfrac{1}{18} i\right) \psi^{-1}\right) a_i a_i \Lambda a_{jj} + \left(\left(\tfrac{1}{18} i\right) \psi^{-1}\right) a_i a_i a_{jj} \Lambda + \\
& \left(\left(-\tfrac{1}{36} i\right) \psi^{-1}\right) a_i a_{jj} \Lambda a_i + \left(\left(-\tfrac{1}{36} i\right) \psi^{-1}\right) a_i a_{jj} a_i \Lambda + \left(\left(-\tfrac{1}{36} i\right) \psi^{-1}\right) a_{ii} \Lambda a_j a_j + \left(\left(-\tfrac{1}{36} i\right) \psi^{-1}\right) a_{ii} a_j \Lambda a_j + \left(\left(-\tfrac{1}{36} i\right) \psi^{-1}\right) a_{ii} a_j a_j \Lambda + \\
& \left(\tfrac{1}{30} i + \left(\tfrac{1}{16} i\right) \psi^{-2}\right) a_i \Lambda a_{ijj} \Lambda + \tfrac{1}{15} i a_i \Lambda a_{jij} \Lambda + \left(\left(-\tfrac{1}{144}\right) \psi^{-1}\right) a_i \Lambda a_i a_j a_j + \left(\tfrac{1}{48} \psi^{-1}\right) a_i \Lambda a_j a_i a_j + \left(\left(-\tfrac{1}{144}\right) \psi^{-1}\right) a_i \Lambda a_j a_j a_i + \\
& \left(\left(-\tfrac{5}{144}\right) \psi^{-1}\right) a_i a_i \Lambda a_j a_j + \left(\left(-\tfrac{1}{144}\right) \psi^{-1}\right) a_i a_i a_j \Lambda a_j + \left(\left(-\tfrac{5}{144}\right) \psi^{-1}\right) a_i a_i a_j a_j \Lambda + \left(\tfrac{1}{48} \psi^{-1}\right) a_i a_j \Lambda a_i a_j + \left(\tfrac{1}{48} \psi^{-1}\right) a_i a_j \Lambda a_j a_i + \\
& \left(\tfrac{1}{48} \psi^{-1}\right) a_i a_j a_i \Lambda a_j + \left(\tfrac{1}{48} \psi^{-1}\right) a_i a_j a_i a_j \Lambda + \left(\left(-\tfrac{1}{144}\right) \psi^{-1}\right) a_i a_j a_j \Lambda a_i + \left(\left(-\tfrac{1}{144}\right) \psi^{-1}\right) a_i a_j a_j a_i \Lambda + \left(-\tfrac{2}{45}\right) a_i \Lambda a_j \Lambda a_{ij} + \left(-\tfrac{2}{45}\right) a_i \Lambda a_j \Lambda a_{ji} +
\end{aligned}$$

$$\left(\frac{1}{45}+\frac{1}{24}\psi^{-2}\right)a_i\Lambda a_j a_{ij}\Lambda+\left(\frac{1}{45}+\left(-\frac{1}{12}\right)\psi^{-2}\right)a_i\Lambda a_j a_{ji}\Lambda+\left(-\frac{1}{45}+\left(-\frac{1}{24}\right)\psi^{-2}\right)a_i\Lambda a_{ij}\Lambda a_j+\left(-\frac{1}{45}+\left(-\frac{1}{24}\right)\psi^{-2}\right)a_i\Lambda a_{ij}a_j\Lambda+$$
$$\left(-\frac{1}{45}+\frac{1}{24}\psi^{-2}\right)a_i\Lambda a_{ji}\Lambda a_j+\left(-\frac{1}{45}+\left(-\frac{1}{12}\right)\psi^{-2}\right)a_i\Lambda a_{ji}a_j\Lambda+\left(\frac{1}{45}+\frac{1}{24}\psi^{-2}\right)a_i a_j\Lambda a_{ij}\Lambda+\left(\frac{1}{45}+\frac{1}{24}\psi^{-2}\right)a_i a_j\Lambda a_{ji}\Lambda+\frac{2}{45}a_i a_{ij}\Lambda a_j\Lambda+$$
$$\left(\frac{2}{45}+\frac{1}{12}\psi^{-2}\right)a_i a_{ji}\Lambda a_j\Lambda+\left(-\frac{2}{45}+\left(-\frac{1}{24}\right)\psi^{-2}\right)a_i\Lambda a_i\Lambda a_{jj}+\frac{1}{45}a_i\Lambda a_i a_{jj}\Lambda+\left(-\frac{1}{45}\right)a_i\Lambda a_{jj}\Lambda a_i+\left(-\frac{1}{45}\right)a_i\Lambda a_{jj}a_i\Lambda+\frac{1}{45}a_i a_i\Lambda a_{jj}\Lambda+$$
$$\left(\frac{2}{45}+\frac{1}{24}\psi^{-2}\right)a_i a_{jj}\Lambda a_i\Lambda+\left(\frac{1}{24}\psi^{-2}\right)a_{ii}\Lambda a_j\Lambda a_j+\left(\left(-\frac{1}{12}\right)\psi^{-2}\right)a_{ii}\Lambda a_j a_j\Lambda+\left(\frac{1}{24}\psi^{-2}\right)a_{ii}a_j\Lambda a_j\Lambda+\left(\frac{1}{120}i+\left(-\frac{5}{192}i\right)\psi^{-2}\right)a_i\Lambda a_i\Lambda a_j a_j+$$
$$\left(\frac{1}{120}i+\left(\frac{1}{64}i\right)\psi^{-2}\right)a_i\Lambda a_i a_j\Lambda a_j+\left(\frac{1}{120}i+\left(-\frac{5}{192}i\right)\psi^{-2}\right)a_i\Lambda a_i a_j a_j\Lambda+\left(\frac{1}{120}i+\left(\frac{1}{64}i\right)\psi^{-2}\right)a_i\Lambda a_j\Lambda a_i a_j+\left(\frac{1}{120}i+\left(\frac{1}{64}i\right)\psi^{-2}\right)a_i\Lambda a_j\Lambda a_j a_i+$$
$$\left(\frac{1}{120}i+\left(\frac{1}{64}i\right)\psi^{-2}\right)a_i\Lambda a_j a_i\Lambda a_j+\left(\frac{1}{120}i+\left(\frac{1}{64}i\right)\psi^{-2}\right)a_i\Lambda a_j a_i a_j\Lambda+\left(\frac{1}{120}i+\left(-\frac{5}{192}i\right)\psi^{-2}\right)a_i\Lambda a_j a_j\Lambda a_i+\left(\frac{1}{120}i+\left(-\frac{5}{192}i\right)\psi^{-2}\right)a_i\Lambda a_j a_j a_i\Lambda+$$
$$\left(\frac{1}{120}i+\left(-\frac{5}{192}i\right)\psi^{-2}\right)a_i a_i\Lambda a_j\Lambda a_j+\left(\frac{1}{120}i+\left(\frac{11}{192}i\right)\psi^{-2}\right)a_i a_i\Lambda a_j a_j\Lambda+\left(\frac{1}{120}i+\left(-\frac{5}{192}i\right)\psi^{-2}\right)a_i a_i a_j\Lambda a_j\Lambda+\left(\frac{1}{120}i+\left(\frac{1}{64}i\right)\psi^{-2}\right)a_i a_j\Lambda a_i\Lambda a_j+$$
$$\left(\frac{1}{120}i+\left(\frac{1}{64}i\right)\psi^{-2}\right)a_i a_j\Lambda a_i a_j\Lambda+\left(\frac{1}{120}i+\left(\frac{1}{64}i\right)\psi^{-2}\right)a_i a_j\Lambda a_j\Lambda a_i+\left(\frac{1}{120}i+\left(\frac{1}{64}i\right)\psi^{-2}\right)a_i a_j\Lambda a_j a_i\Lambda+\left(\frac{1}{120}i+\left(\frac{1}{64}i\right)\psi^{-2}\right)a_i a_j a_i\Lambda a_j\Lambda+$$
$$\left(\frac{1}{120}i+\left(-\frac{5}{192}i\right)\psi^{-2}\right)a_i a_j a_j\Lambda a_i\Lambda+\left(\left(\frac{1}{18}i\right)\psi^{-1}\right)a_i\Lambda a_j\Lambda a_{ij}\Lambda+\left(\left(\frac{1}{18}i\right)\psi^{-1}\right)a_i\Lambda a_j\Lambda a_{ji}\Lambda+\left(\left(-\frac{1}{18}i\right)\psi^{-1}\right)a_i\Lambda a_{ij}\Lambda a_j\Lambda+$$
$$\left(\left(\frac{1}{9}i\right)\psi^{-1}\right)a_i\Lambda a_{ji}\Lambda a_j\Lambda+\left(\left(-\frac{1}{36}i\right)\psi^{-1}\right)a_i\Lambda a_i\Lambda a_{jj}\Lambda+\left(\left(\frac{1}{36}i\right)\psi^{-1}\right)a_i\Lambda a_{jj}\Lambda a_i\Lambda+\left(\left(\frac{1}{12}i\right)\psi^{-1}\right)a_{ii}\Lambda a_j\Lambda a_j\Lambda+\left(\left(-\frac{1}{48}\right)\psi^{-1}\right)a_i\Lambda a_i\Lambda a_j\Lambda a_j+$$
$$\left(\frac{1}{16}\psi^{-1}\right)a_i\Lambda a_i\Lambda a_j a_j\Lambda+\left(\left(-\frac{1}{48}\right)\psi^{-1}\right)a_i\Lambda a_i a_j\Lambda a_j\Lambda+\left(\left(-\frac{1}{48}\right)\psi^{-1}\right)a_i\Lambda a_j\Lambda a_i\Lambda a_j+\left(\left(-\frac{1}{48}\right)\psi^{-1}\right)a_i\Lambda a_j\Lambda a_i a_j\Lambda+\left(\left(-\frac{1}{48}\right)\psi^{-1}\right)a_i\Lambda a_j\Lambda a_j\Lambda a_i+$$
$$\left(\left(-\frac{1}{48}\right)\psi^{-1}\right)a_i\Lambda a_j\Lambda a_j a_i\Lambda+\left(\left(-\frac{1}{48}\right)\psi^{-1}\right)a_i\Lambda a_j a_i\Lambda a_j\Lambda+\left(\frac{1}{16}\psi^{-1}\right)a_i\Lambda a_j a_j\Lambda a_i\Lambda+\left(\frac{1}{16}\psi^{-1}\right)a_i a_i\Lambda a_j\Lambda a_j\Lambda+\left(\left(-\frac{1}{48}\right)\psi^{-1}\right)a_i a_j\Lambda a_i\Lambda a_j\Lambda+$$
$$\left(\left(-\frac{1}{48}\right)\psi^{-1}\right)a_i a_j\Lambda a_j\Lambda a_i\Lambda+\left(-\frac{1}{24}i+\left(-\frac{1}{64}i\right)\psi^{-2}\right)a_i\Lambda a_i\Lambda a_j\Lambda a_j\Lambda+\left(-\frac{1}{24}i+\left(-\frac{1}{64}i\right)\psi^{-2}\right)a_i\Lambda a_j\Lambda a_i\Lambda a_j\Lambda+\left(-\frac{1}{24}i+\left(-\frac{1}{64}i\right)\psi^{-2}\right)a_i\Lambda a_j\Lambda a_j\Lambda a_i\Lambda$$

### F. Trace permutation and integration by parts

So we define "canonicalization" for the terms. We already defined an ordering of the monomials, so we can permute cyclically under trace and relabel, and pick the unique minimal monomial:

**Code 10** (Trace permutation)**.**

```
@distributive_op
def tr_permute(m, c, algebra):
    return min((relabel(algebra.term(GG(m.value[k:] + m.value[:k]), c)) for k in range(len(m))),
               default=algebra.term(m, c))
```

For integration by parts, we integrate a factor by parts if this generates only smaller monomials, with trace permutation applied before and after. (For later use, we also consider indices on some variables to be covariant derivatives.)

**Code 11** (Integration by parts under trace)**.**

```
@distributive_op
def integrate_by_parts(m, c, algebra, covariant=False, max_key=None):
    if max_key is None:
        max_key = lambda m: m

    m = tr_permute(m)

    res = algebra.term(m, c)
    max_m = max_key(m)

    for k, (letter, idx) in enumerate(m.value):
        if (not idx or letter == "a" and len(idx) <= 1 or
                letter in ("F", "delta") and len(idx) <= 2 or
                letter in ("V") and len(idx) <= 1):
            continue

        try:
            _check_diff(letter, idx, covariant)
            m2 = algebra.term(GG([(letter, idx[:-1])]), -c)
            new = deriv_R(algebra(m[k+1:] * m[:k]), idx[-1], covariant=covariant) * m2
        except DifferentiationError:
            break

        if all(max_key(m2) < max_m for m2, c2 in new):
            res = new
            if not res:
                break
```

```
            max_m = max(max_key(m2) for m2, c2 in res)

        return tr_permute(res)

    def integrate_by_parts_all(expr, covariant=False, max_key=None):
        prev_expr = 0
        while expr != prev_expr:
            prev_expr = expr
            expr = integrate_by_parts(expr, max_key=max_key, covariant=covariant)
        return expr
```

For example (again, dummy summation and trace implied):

$$a_i a_{ijj} \mapsto (-1)\, a_{ij} a_{ij}\,, \quad a_i a_i a_{jj} \mapsto (-1)\, a_i a_j a_{ij} + (-1)\, a_i a_j a_{ji}\,. \tag{29}$$

We also do a few integrations by parts the above rule does not cover: $X a_{ii} Y a_{jj} \mapsto -X a_{iij} Y a_j = -X a_{iji} Y a_j \mapsto X a_{ij} Y a_{ji}$ where $X$, $Y$ are constant:

**Code 12** (Special integration by parts)**.**

```
    def ip_manual(expr):
        # Manual special cases:
        cases = [
            (a('ii')*a('jj'), a('ij')*a('ji')),
            (Lambda*a('ii')*a('jj'), Lambda*a('ij')*a('ji')),
            (Lambda*a('ii')*Lambda*a('jj'), Lambda*a('ij')*Lambda*a('ji')),
        ]
        for f1, f2 in cases:
            expr = expr - expr.coefficient(GG(f1)) * (f1 - f2)
        return expr
```

```
avg_log_2_p = integrate_by_parts(avg_log_2)
avg_log_4_p = ip_manual(integrate_by_parts(integrate_by_parts(avg_log_4)))
```

$\texttt{avg\_log\_2\_p} = \left(-\frac{1}{6} i\right) a_i a_i + \frac{1}{6} i \Lambda a_i \Lambda a_i$

$\texttt{avg\_log\_4\_p} = \left(\frac{1}{30} i + \left(\frac{1}{16} i\right) \psi^{-2}\right) a_{ij} a_{ij} + \frac{1}{15} i a_{ij} a_{ji} + \left(\left(-\frac{1}{8}\right) \psi^{-2}\right) a_i a_j a_{ij} + \left(\frac{1}{8} \psi^{-2}\right) a_i a_j a_{ji} + \left(-\frac{1}{60} i + \left(\frac{3}{32} i\right) \psi^{-2}\right) a_i a_i a_j a_j + \left(-\frac{1}{120} i + \left(-\frac{5}{64} i\right) \psi^{-2}\right) a_i a_j a_i a_j + \left(\left(-\frac{1}{12} i\right) \psi^{-1}\right) \Lambda a_i a_j a_{ij} + \left(\left(\frac{1}{12} i\right) \psi^{-1}\right) \Lambda a_i a_j a_{ji} + \left(\left(-\frac{1}{12} i\right) \psi^{-1}\right) \Lambda a_i a_{ij} a_j + \left(\left(\frac{1}{12} i\right) \psi^{-1}\right) \Lambda a_i a_{ji} a_j + \left(-\frac{1}{30} i + \left(-\frac{1}{16} i\right) \psi^{-2}\right) \Lambda a_{ij} \Lambda a_{ij} + \left(-\frac{1}{15} i\right) \Lambda a_{ij} \Lambda a_{ji} + \left(\left(-\frac{1}{12} i\right) \psi^{-1}\right) \Lambda a_{ij} a_i a_j + \left(\left(\frac{1}{12} i\right) \psi^{-1}\right) \Lambda a_{ij} a_j a_i + \left(\left(-\frac{1}{12}\right) \psi^{-1}\right) \Lambda a_i a_i a_j a_j + \left(\frac{1}{12} \psi^{-1}\right) \Lambda a_i a_j a_i a_j + \left(\frac{2}{15} + \frac{1}{8} \psi^{-2}\right) \Lambda a_i \Lambda a_j a_{ij} + \frac{1}{15} \Lambda a_i \Lambda a_j a_{ji} + \left(-\frac{2}{15} + \left(-\frac{1}{8}\right) \psi^{-2}\right) \Lambda a_i \Lambda a_{ij} a_j + \left(-\frac{1}{15}\right) \Lambda a_i \Lambda a_{ji} a_j + \left(-\frac{1}{15}\right) \Lambda a_i a_j \Lambda a_{ij} + \frac{1}{15} \Lambda a_i a_j \Lambda a_{ji} + \left(\frac{1}{30} i + \left(-\frac{1}{16} i\right) \psi^{-2}\right) \Lambda a_i \Lambda a_i a_j a_j + \left(\frac{1}{30} i + \left(\frac{1}{16} i\right) \psi^{-2}\right) \Lambda a_i \Lambda a_j a_i a_j + \left(\frac{1}{30} i + \left(-\frac{1}{16} i\right) \psi^{-2}\right) \Lambda a_i \Lambda a_j a_j a_i + \left(\frac{1}{60} i + \left(\frac{1}{32} i\right) \psi^{-2}\right) \Lambda a_i a_i \Lambda a_j a_j + \left(\frac{1}{60} i + \left(\frac{1}{32} i\right) \psi^{-2}\right) \Lambda a_i a_j \Lambda a_i a_j + \left(\frac{1}{60} i + \left(\frac{1}{32} i\right) \psi^{-2}\right) \Lambda a_i a_j \Lambda a_j a_i + \left(\left(\frac{1}{12} i\right) \psi^{-1}\right) \Lambda a_i \Lambda a_j \Lambda a_{ij} + \left(\left(-\frac{1}{12} i\right) \psi^{-1}\right) \Lambda a_i \Lambda a_j \Lambda a_{ji} + \left(\frac{1}{6} \psi^{-1}\right) \Lambda a_i \Lambda a_i \Lambda a_j a_j + \left(\left(-\frac{1}{12}\right) \psi^{-1}\right) \Lambda a_i \Lambda a_i a_j \Lambda a_j + \left(\left(-\frac{1}{12}\right) \psi^{-1}\right) \Lambda a_i \Lambda a_j \Lambda a_i a_j + \left(-\frac{1}{12} i + \left(-\frac{1}{32} i\right) \psi^{-2}\right) \Lambda a_i \Lambda a_i \Lambda a_j \Lambda a_j + \left(-\frac{1}{24} i + \left(-\frac{1}{64} i\right) \psi^{-2}\right) \Lambda a_i \Lambda a_j \Lambda a_i \Lambda a_j$

We can here note that expansions with $\mathcal{G}$ first or last inside the logarithm are identical after these operations:

```
X_4_rev, log_4_rev, avg_log_4_rev = gradient_expansion(max_order=4, reverse=True)
avg_log_4_rev = avg_log_4_rev - avg_log_2_a
```

$\texttt{ip\_manual(integrate\_by\_parts\_all(avg\_log\_4} - \texttt{avg\_log\_4\_rev))} = 0$

Finally, pick the leading term for $p_F \ell \gg 1$, which is $\propto \psi^0$:

```
avg_log_4_leading = avg_log_4_p.map_coefficients(lambda c: c.monomial_coefficient(PP(1)))
```

$\texttt{avg\_log\_4\_leading} =$
$\frac{1}{30} i a_{ij} a_{ij} + \frac{1}{15} i a_{ij} a_{ji} - \frac{1}{60} i a_i a_i a_j a_j - \frac{1}{120} i a_i a_j a_i a_j - \frac{1}{30} i \Lambda a_{ij} \Lambda a_{ij} - \frac{1}{15} i \Lambda a_{ij} \Lambda a_{ji} + \frac{2}{15} \Lambda a_i \Lambda a_j a_{ij} + \frac{1}{15} \Lambda a_i \Lambda a_j a_{ji} - \frac{2}{15} \Lambda a_i \Lambda a_{ij} a_j - \frac{1}{15} \Lambda a_i \Lambda a_{ji} a_j - \frac{1}{15} \Lambda a_i a_j \Lambda a_{ij} + \frac{1}{15} \Lambda a_i a_j \Lambda a_{ji} + \frac{1}{30} i \Lambda a_i \Lambda a_i a_j a_j + \frac{1}{30} i \Lambda a_i \Lambda a_j a_i a_j + \frac{1}{30} i \Lambda a_i \Lambda a_j a_j a_i + \frac{1}{60} i \Lambda a_i a_i \Lambda a_j a_j + \frac{1}{60} i \Lambda a_i a_j \Lambda a_i a_j + \frac{1}{60} i \Lambda a_i a_j \Lambda a_j a_i - \frac{1}{12} i \Lambda a_i \Lambda a_i \Lambda a_j \Lambda a_j - \frac{1}{24} i \Lambda a_i \Lambda a_j \Lambda a_i \Lambda a_j$

This should then be rewritten in covariant form, but it's hard to do by hand.

### G. Covariant form

Reduction to covariant form is done as explained in the Appendix of the main text. We implement it as follows:

**Code 13** (General noncommutative reduction under trace + covariant form)**.**

```
def divide_monomial_cyclic(m1, m2):
    """Yield (d, 1) such that m1 = d*m2 (mod cyclic permutation), if it exists, otherwise None"""
    if len(m2.value) == 0:
        yield (m1, GG.one())
        return
    elif len(m1.value) < len(m2.value):
        return

    for k in range(len(m1.value)):
        end = (k + len(m2.value)) % len(m1.value)
        if k < end and m2.value == m1.value[k:end]:
            yield GG(m1.value[end:] + m1.value[:k]), GG.one()
        elif end <= k and m2.value == m1.value[k:] + m1.value[:end]:
            yield GG(m1.value[end:k]), GG.one()

def divide_monomial(m1, m2):
    """Yield (l, r) such that m1 = l*m2*r, if it exists, otherwise None"""
    if len(m2.value) == 0:
        yield (m1, GG.one())
        return
    for k in range(0, len(m1.value) - len(m2.value) + 1):
        if m1.value[k:k+len(m2.value)] == m2.value:
            yield GG(m1.value[:k]), GG(m1.value[k+len(m2.value):])

def max_degree(expr):
    return max((len(m) for m in expr.monomial_coefficients()), default=0)

def reduce_term(expr, ideal, max_key=None, max_deg=None, disp=False, simplify=tr_permute,
                divide=divide_monomial_cyclic):
    # Computations in QQi are faster, so try it
    (expr, *ideal), orig_algebra = try_coerce_algebra(expr, *ideal, to=GG.algebra(QQi))

    if (hasattr(expr.base_ring(), 'element_class') and
            hasattr(expr.base_ring().element_class, 'monomial_coefficient')):
        # Separate computation for each coef monomial (again, faster)
        toalg = lambda z: coerce_algebra(z, GG.algebra(QQi))
        fromalg = lambda z: coerce_algebra(z, FF)
        pp_mons = sorted(set(m for cc in expr.coefficients() for m in PP(cc).monomials()))
        ideal = [toalg(el) for el in ideal]
        terms = [toalg(expr.map_coefficients(lambda z: PP(z).monomial_coefficient(m)))
                 for m in pp_mons]
        args = (ideal, max_key, max_deg, disp, simplify, divide)
        expr = sum(fromalg(_reduce_term(t, *args)).map_coefficients(lambda z: PP(m)*PP(z))
                   for m, t in zip(pp_mons, terms))
    else:
        expr = _reduce_term(expr, ideal, max_key, max_deg, disp, simplify, divide)

    return coerce_algebra(expr, orig_algebra)

def _reduce_term(expr, ideal, max_key, max_deg, disp, simplify, divide):
    # Actual computations

    expr = simplify(expr)

    if max_key is not None:
        max_key_c = lambda v: (max_key(v[0]),) + v[1:]
```

```
    else:
        max_key_c = None

    if max_deg is None:
        max_deg = max_degree(expr)
    elif max_deg < 0:
        max_deg = max_degree(expr) - max_deg

    algebra = expr.parent()
    ring = algebra.base_ring()

    # Find ideal elements whose monomial cyclic-divides monomials in *expr*.
    # Complete the monomial set iterative up to degree bound.
    factors = set()
    monomials = set()
    new_monomials = list(expr.monomial_coefficients())
    while new_monomials:
        m = new_monomials.pop()
        if m in monomials:
            continue
        monomials.add(m)
        for el in ideal:
            for el_m, el_c in el:
                for lpart, rpart in divide(m, el_m):
                    r = simplify((1 / el_c) * algebra(lpart) * el * algebra(rpart))
                    if max_degree(r) <= max_deg:
                        factors.add(r)
                        new_monomials.extend(r.monomial_coefficients())

    if factors:
        # Gaussian elimination on factors.
        # Convert to matrix problem, solve, and convert back.
        monomials = sorted(monomials, key=max_key, reverse=True)
        mat = matrix(ring, [[f.coefficient(m) for m in monomials] for f in factors])
        if disp:
            print(f"BASIS: {monomials}")
            print(f"MAT:\n{mat}")
        mat.echelonize()
        factors = [algebra.sum_of_terms(zip(monomials, row))
                   for row in mat.rows() if any(row)]

    # Reduce expr against factors
    for f in factors:
        if disp:
            print(f"REDUCED FACTOR: {f}")
        f_m, f_c = max(f, key=max_key_c)
        expr_c = expr.coefficient(f_m)
        if expr_c != 0:
            expr -= expr_c/f_c * f

    return expr

def to_covariant(expr, max_deg=None, disp=False):
    # Note: it only needs the defining relations as input, rest is inferred!
    # Our monomial matching however doesn't know about index permutations,
    # so we need to list them all here.
    comm = lambda a, b: a*b - b*a
    ideal = [rule for i, j in Permutations("ij") for rule in [
        comm(-I * a(i), Lambda) - Q(i),
        comm(-I * a(j), Q(i)) + comm(-I*a((i,j)), Lambda) - Q((i,j)),
        a((j,i)) - a((i,j)) - I*comm(a(i), a(j)) - F((i,j)),
        F((j,i)) + F((i,j)),
```

```
        ]]
        return reduce_term(expr, ideal, _max_key, max_deg=max_deg, disp=disp)

    def _max_key(m):
        cov_badness = sum(letter in ("a",) for letter, idx in m.value)
        return (cov_badness, m)

    def coerce_algebra(expr, algebra):
        if expr.parent().indices() != algebra.indices(): raise TypeError("incompatible basis")
        ring = algebra.base_ring()
        try:
            return algebra.sum_of_terms((m, ring(c)) for m, c in expr)
        except TypeError:
            return algebra.sum_of_terms((m, ring(SR(c))) for m, c in expr)

    def try_coerce_algebra(*args, to=None):
        try:
            return tuple(coerce_algebra(arg, to) for arg in args), args[0].parent()
        except (TypeError, NotImplementedError):
            return args, args[0].parent()
```

Some nontrivial examples (under trace as always):

$$\texttt{to\_covariant}(Q_i\Lambda Q_i Q_j a_j, \texttt{max\_deg} = 6) = \left(-\frac{1}{2}i\right) Q_i Q_i Q_j Q_j \tag{30}$$

$$\begin{aligned}\texttt{to\_covariant}(&(-1)\, a_i a_j a_{ij} + a_i a_j a_{ji} + i a_i a_i a_j a_j + (-i)\, a_i a_j a_i a_j + \Lambda a_i \Lambda a_j a_{ij} + \\ &(-1)\, \Lambda a_i \Lambda a_j a_{ji} + (-1)\, \Lambda a_i \Lambda a_{ij} a_j + \Lambda a_i \Lambda a_{ji} a_j + (-1)\, \Lambda a_i a_j \Lambda a_{ij} + \\ &\Lambda a_i a_j \Lambda a_{ji} + (-i)\, \Lambda a_i \Lambda a_i a_j a_j + 2i \Lambda a_i \Lambda a_j a_i a_j + (-i)\, \Lambda a_i \Lambda a_j a_j a_i + \\ &(-i)\, \Lambda a_i a_j \Lambda a_i a_j + i \Lambda a_i a_j \Lambda a_j a_i) = F_{ij} Q_i Q_j\end{aligned} \tag{31}$$

Finally, applying the above procedure to the results obtained above, we find:

```
avg_log_2_p_cov = to_covariant(avg_log_2_p)
avg_log_4_leading_cov = to_covariant(avg_log_4_leading)
```

$$\texttt{avg\_log\_2\_p\_cov} = \left(-\frac{1}{12}i\right) Q_i Q_i\,, \tag{32}$$

$$\texttt{avg\_log\_4\_leading\_cov} = \tfrac{1}{60} i Q_{ij} Q_{ij} + \tfrac{1}{30} i Q_{ij} Q_{ji} + \tfrac{1}{30} F_{ij} Q_i Q_j + \left(-\tfrac{1}{24} i\right) Q_i Q_i Q_j Q_j + \left(-\tfrac{1}{48} i\right) Q_i Q_j Q_i Q_j \quad . \tag{33}$$

That the expression above is equal to where we started from can be verified:

```
acomm = lambda a, b: a*b+b*a
comm = lambda a, b: a*b-b*a
Qival = comm(-I*a('i'), Lambda)
Qjval = comm(-I*a('j'), Lambda)
Qijval = comm(-I*a('ij'), Lambda) + comm(-I*a('j'), Qival)
Qjival = comm(-I*a('ji'), Lambda) + comm(-I*a('i'), Qjval)
Fijval = a('ji') - a('ij') - I*comm(a('i'), a('j'))
Fjival = -Fijval

avg_log_4_manual = (I/60 * Qijval*Qijval + I/30*Qijval*Qjival + 1/30*Qival*Qjval*Fijval
                    - I/24*Qival*Qival*Qjval*Qjval - I/48*Qival*Qjval*Qival*Qjval)

diff_vs_manual = tr_permute(avg_log_4_manual - avg_log_4_leading)
```

$$\texttt{diff\_vs\_manual} = 0\,. \tag{34}$$

### H. Next orders in $p_F \ell$

As the above procedure is automatic, we can as well compute the next orders in the $\psi = p_F \ell$ expansion.

```
avg_log_4_psi2 = avg_log_4_p.map_coefficients(lambda c: c.monomial_coefficient(psi**-1))
avg_log_4_psi1 = avg_log_4_p.map_coefficients(lambda c: c.monomial_coefficient(psi**-2))
```

avg_log_4_psi2 $=$
$-\frac{1}{12} i\Lambda a_i a_j a_{ij} + \frac{1}{12} i\Lambda a_i a_j a_{ji} - \frac{1}{12} i\Lambda a_i a_{ij} a_j + \frac{1}{12} i\Lambda a_i a_{ji} a_j - \frac{1}{12} i\Lambda a_{ij} a_i a_j + \frac{1}{12} i\Lambda a_{ij} a_j a_i - \frac{1}{12} \Lambda a_i a_i a_j a_j + \frac{1}{12} \Lambda a_i a_j a_i a_j + \frac{1}{12} i\Lambda a_i \Lambda a_j \Lambda a_{ij} - \frac{1}{12} i\Lambda a_i \Lambda a_j \Lambda a_{ji} + \frac{1}{6} \Lambda a_i \Lambda a_i \Lambda a_j a_j - \frac{1}{12} \Lambda a_i \Lambda a_i a_j \Lambda a_j - \frac{1}{12} \Lambda a_i \Lambda a_j \Lambda a_i a_j$
avg_log_4_psi1 $= \frac{1}{16} i a_{ij} a_{ij} - \frac{1}{8} a_i a_j a_{ij} + \frac{1}{8} a_i a_j a_{ji} + \frac{3}{32} i a_i a_i a_j a_j - \frac{5}{64} i a_i a_j a_i a_j - \frac{1}{16} i\Lambda a_{ij} \Lambda a_{ij} + \frac{1}{8} \Lambda a_i \Lambda a_j a_{ij} - \frac{1}{8} \Lambda a_i \Lambda a_{ij} a_j - \frac{1}{16} i\Lambda a_i \Lambda a_i a_j a_j + \frac{1}{16} i\Lambda a_i \Lambda a_j a_i a_j - \frac{1}{16} i\Lambda a_i \Lambda a_j a_j a_i + \frac{1}{32} i\Lambda a_i a_i \Lambda a_j a_j + \frac{1}{32} i\Lambda a_i a_j \Lambda a_i a_j + \frac{1}{32} i\Lambda a_i a_j \Lambda a_j a_i - \frac{1}{32} i\Lambda a_i \Lambda a_i \Lambda a_j \Lambda a_j - \frac{1}{64} i\Lambda a_i \Lambda a_j \Lambda a_i \Lambda a_j$

We'll also now change notation by introducing $T(\ldots)T^{-1}$ inside the trace, which transforms $\Lambda \mapsto Q$, and removes the extra factors of $T$ in the definitions of $Q_i$, $Q_{ij}$, $F_{ij}$ reducing them directly to usual covariant derivatives and the usual field strength.

```
@distributive_op
def lambda_to_Q(m, c, algebra):
    ltrmap = {"Lambda": "Q"}
    return [([(ltrmap.get(letter, letter), idx) for letter, idx in m.value], c)]

avg_log_4_psi2_cov = lambda_to_Q(to_covariant(avg_log_4_psi2))
avg_log_4_psi1_cov = lambda_to_Q(to_covariant(avg_log_4_psi1))
```

avg_log_4_psi2_cov $= \frac{1}{12} Q Q_{ij} Q_{ij} + \frac{1}{12} i F_{ij} Q Q_i Q_j$
avg_log_4_psi1_cov $= \frac{1}{32} i Q_{ij} Q_{ij} + \frac{1}{16} F_{ij} Q_i Q_j + \left(-\frac{1}{64} i\right) Q_i Q_i Q_j Q_j + \left(-\frac{1}{128} i\right) Q_i Q_j Q_i Q_j$

Note that all orders in the $\psi = p_F \ell$ have to be expressible in a covariant form, and this indeed comes out.

Similarly as above, we can check the above covariant expressions are equal to the values expressed in terms of $\Lambda$ and $a$:

```
Qval = Lambda
avg_log_4_psi2_manual = (1/12 * Qval*Qijval*Qijval + I/12*Fijval*Qval*Qival*Qjval)
avg_log_4_psi1_manual = (I/32*Qijval*Qijval + 1/16*Fijval*Qival*Qjval
                         - I/64*Qival*Qival*Qjval*Qjval - I/128*Qival*Qjval*Qival*Qjval)
diff_vs_manual_psi2 = tr_permute(avg_log_4_psi2_manual - avg_log_4_psi2)
diff_vs_manual_psi1 = tr_permute(avg_log_4_psi1_manual - avg_log_4_psi1)
```

$$\texttt{diff\_vs\_manual\_psi2} = 0\,, \qquad \texttt{diff\_vs\_manual\_psi1} = 0\,. \tag{35}$$

### I. Symmetrization

The above forms are a bit ambiguous: higher-order derivatives because of $[\hat{\nabla}_i, \hat{\nabla}_j] = [-iF_{ij}, \cdot]$, and the results can also be covariantly integrated by parts, because $\int \mathrm{d}R \,\mathrm{tr}\, \hat{\nabla}_i X = \int \mathrm{d}R \,(\partial_i \,\mathrm{tr}\, X - i\,\mathrm{tr}[A_i, X]) = 0$ (as before, we neglect total derivative terms) and $\hat{\nabla}_i(XY) = (\hat{\nabla}_i X)Y + X(\hat{\nabla}_i Y)$. To try to find a less ambiguous form, we can rewrite the above in terms of the symmetrized derivatives $Q_{(i_1 \ldots i_n)} := \frac{1}{|\mathcal{P}|}\sum_{\sigma\in\mathcal{P}} Q_{\sigma(i_1)\ldots\sigma(i_n)}$, which are the average over all index permutations. We can do this in a similar reduction we did to get the covariant form:

**Code 14** (Conversion to symmetrized derivatives.)**.**

```
def to_Q_symmetrized(expr):
    return reduce_term(expr, Q_ideal(sym=True), max_deg=-2, max_key=_max_key_Q, simplify=_cov_Q_ip)

def _max_key_Q(m):
    # Prefer to not have higher derivatives of Q in the result
```

```
    Qcount = sum((1 if v.letter == "Q" and len(v.idx) > 1 and ";" not in v.idx else 0) for v in m)
    has_F = any(v.letter == "F" for v in m)
    Qscount = sum(1 if v.letter == "Q" and ";" in v.idx else 0 for v in m)
    Qdercount = sum(1 if (v.letter == "Q" and v.idx and ";" not in v.idx) else 0 for v in m)
    if Qdercount > 0 and Qscount > 0 or Qscount > 1:
        Qcount += 10
    return (Qcount, len(m), m)

def _cov_Q_ip(expr):
    return integrate_by_parts_all(expr, covariant=True)

def Q_ideal(sym=False, with_F=True, idxs="ij"):
    # Basic commutation rules and definitions
    ideal = [Q()*Q(i) + Q(i)*Q() for i in idxs]
    if with_F:
        ideal += [
            F("ij") + F("ji"),
            F("i0") + F("0i"),
        ]
        # [D_i, D_j] X = [-i F_ij, X]
        ideal += [sym(base + "ji") - sym(base + "ij") - comm(-I*F("ij"), sym(base))
                  for sym, base in cartesian_product_iterator([[Q, f], ["", "i", "j", "ij", "ji"]])]
        ideal += [sym("0i") - sym("i0") - comm(-I*F("i0"), sym()) for sym in [Q, f]]
    ideal = ideal_deriv_R(ideal, idxs=idxs)
    if not sym:
        return ideal
    # Definitions of the symmetrized indices
    ideal += [
        sum(v(z) for z in Permutations(P)) - len(Permutations(P))*vs(P)
        for P in ["ij", "iij", "ijj", "iijj", "ii", "jj", "i0"]
        for v, vs in [(Q, Qs), (f, fs)]
    ]
    # Definitions of 2-term symmetrization
    ideal += [
        sum(v(z[0])*v(z[1:]) for z in Permutations(P)) - len(Permutations(P)) * vs(P[0]+";"+P[1:])
        for P in ["ij", "i0", "ij0", "ii0", "iij", "ijj"]
        for v, vs in [(Q, Qs), (f, fs)]
    ]
    ideal += [
        sum(v(z[:2])*v(z[2:]) for z in Permutations(P)) - len(Permutations(P)) * vs(P[:2]+";"+P[2:])
        for P in ["iijj", "ijj"]
        for v, vs in [(Q, Qs), (f, fs)]
    ]
    # Definitions of 3-term symmetrization
    ideal += [
        sum(v(z[0])*v(z[1])*v(z[2:]) for z in Permutations(P))
        - len(Permutations(P)) * vs(P[0]+";"+P[1]+";"+P[2:])
        for P in ["iijj", "ijj"]
        for v, vs in [(Q, Qs), (f, fs)]
    ]
    # Definitions of 4-term symmetrization
    ideal += [
        sum(v(z[0])*v(z[1])*v(z[2])*v(z[3]) for z in Permutations(P))
        - len(Permutations(P)) * vs(";".join(P))
        for P in ["iijj"]
        for v, vs in [(Q, Qs), (f, fs)]
    ]
    return ideal

def ideal_deriv_R(ideal, idxs="ij"):
    """Add generators to ideal by taking derivatives"""
    # Generate derivatives, with at most 2 of each index
```

```
    ideal = list(ideal)
    items = ideal
    while items:
        new = []
        for expr in items:
            for i in idxs:
                expr2 = deriv_R(expr, i, covariant=True)
                max_count = max(sum(v.idx.count(j) for v in m)
                                for m, c in expr2 for v in m for j in v.idx)
                if max_count <= 2:
                    new.append(expr2)
        ideal += new
        items = new
    return ideal
```

Applying this to the above, we get

$$\delta S_{4,0} = \frac{-\pi\nu_F}{2}\ell^4\tau^{-1}\,\mathrm{Tr}\Big\{\frac{1}{20}iQ_{(ii}Q_{jj)} + \left(-\frac{1}{16}i\right)Q_{(i}Q_iQ_jQ_{j)}\Big\}\,, \tag{36}$$

$$\delta S_{4,1} = \frac{-\pi\nu_F}{2}\ell^4\tau^{-1}\,\mathrm{Tr}\Big\{\left(-\frac{1}{12}\right)Q_iQ_jQ_{ij} + \frac{1}{12}iF_{ij}QQ_iQ_j\Big\}\,, \tag{37}$$

Above, $\mathrm{tr}\,Q_{(ii}Q_{jj)} = \frac{1}{3}\,\mathrm{tr}(Q_{ii}Q_{jj} + Q_{ij}Q_{ji} + Q_{ij}Q_{ij})$ and $\mathrm{tr}\,Q_{(i}Q_iQ_jQ_{j)} = \frac{1}{3}\,\mathrm{tr}(2Q_iQ_iQ_jQ_j + Q_iQ_jQ_iQ_j)$ mean symmetrization across the full index set between braces. The $\delta S_{4,0}$ term then is similar to a symmetrized $c_1(\partial^2 Q)^2 + c_2(\partial Q)^4$.

## J. Expansion with $a_0$

We'll now obtain the $a_0$ terms of the expansion. We will here show results for $d = 3$.

```
@distributive_op
def pick_a0(m, c, algebra):
    has_0 = any("0" in idx for letter, idx in m.value)
    return [(m, c)] if has_0 else []
```

The terms not containing $a_0$ we discussed in previous subsections, and need not be written here.

First, second order, doing the transformations we have discussed earlier:

```
X_2_a0, log_2_a0, avg_log_2_a0 = gradient_expansion(max_order=2, with_a0=True, igorder=0, ndim=3)
avg_log_2_a0low = integrate_by_parts(pick_a0(avg_log_2_a0))
```

$$\begin{aligned}\texttt{avg\_log\_2\_a0} = {}& C_{010}a_0 + \left(\tfrac{1}{6} + \left(\tfrac{1}{3}i\right)\psi^{-1}C_{120}\right)a_{ii} + a_0\Lambda + \left(-\tfrac{1}{2}i\right)a_0a_0 + \\ & \left(\left(-\tfrac{1}{2}\right)\psi^{-1}C_{010} + \left(-\tfrac{1}{3}\right)\psi^{-1}C_{120}\right)a_ia_i + \left(\left(-\tfrac{1}{2}i\right)\psi^{-1}\right)a_{ii}\Lambda + \left(\tfrac{1}{4}\psi^{-1}\right)a_0\Lambda a_0 + \\ & \left(\tfrac{1}{4}\psi^{-1}\right)a_0a_0\Lambda + \left(\tfrac{1}{4}\psi^{-1}\right)a_i\Lambda a_i + \left(\left(-\tfrac{1}{4}\right)\psi^{-1}\right)a_ia_i\Lambda + \tfrac{1}{2}ia_0\Lambda a_0\Lambda + \tfrac{1}{6}ia_i\Lambda a_i\Lambda\end{aligned}\quad , \tag{38}$$

$$\texttt{avg\_log\_2\_a0low} = C_{010}a_0 + \Lambda a_0 + \left(-\tfrac{1}{2}i\right)a_0a_0 + \left(\tfrac{1}{2}\psi^{-1}\right)\Lambda a_0a_0 + \tfrac{1}{2}i\Lambda a_0\Lambda a_0 \quad , \tag{39}$$

We rewrite this to a "covariant" form using also the additional relations from Sec. III.G concerning the "0" index:

**Code 15.**

```
def to_covariant_lambda0(expr, max_deg=None, disp=False):
    ideal = lambda0_ideal()
    return reduce_term(expr, ideal, _max_key_lambda0, max_deg=max_deg, disp=disp)
```

```
def lambda0_ideal():
    comm = lambda a, b: a*b - b*a
    ideal = [rule for i in "ij" for j in "ij" for rule in [
        comm(-I * a(i), Lambda) - Q(i),
        comm(-I * a(j), Q(i)) + comm(-I*a((i,j)), Lambda) - Q((i,j)),
        a((j,i)) - a((i,j)) - I*comm(a(i), a(j)) - F((i,j)),
        F((j,i)) + F((i,j)),
    ]]
    ideal += [
        comm(-I * a("0"), Lambda) - Q("0"),
    ]
    ideal += [rule for nu in "0ij" for rule in [
        comm(-I * a("0"), Q(nu)) - Q((nu, "0")),
    ]]
    ideal += [rule for i in "ij" for rule in [
        a(("0",i)) - I*comm(a(i), a("0")) - F((i,"0")),
        F(("0",i)) + F((i,"0")),
    ]]
    ideal += [rule for i in "ij" for rule in [
        Q((i, "0")) + comm(-I*F((i, "0")), Lambda) - Q(("0", i))
    ]]
    return ideal

def _max_key_lambda0(m):
    # Prefer to eliminate all a, and have maximum F
    cov_spat_badness = sum(letter in ("a",) and "0" not in idx for letter, idx in m.value)
    cov_badness = sum(letter in ("a",) for letter, idx in m.value)
    fcount = sum(letter in ("F",) for letter, idx in m.value)
    qi0count = sum(1 for letter, idx in m.value
                   if letter == "Q" and idx[:1] != ("0",) and "0" in idx)
    return (cov_spat_badness, cov_badness, -fcount, qi0count, m)
```

Hence, with the notation of Sec. III.G for the "0-derivatives", $Q_{\dots,0} := T^{-1}[-i(\mathcal{E} + A_0), Q_{\dots}]T$, we can write

$$\texttt{avg\_log\_2\_a0low} \mapsto C_{010}a_0 + \Lambda a_0 + \left(-\tfrac{1}{4}i\right) Q_0Q_0 + \left(\tfrac{1}{2}\psi^{-1}\right)\Lambda a_0a_0 \tag{40}$$

We can now go to the fourth order in the expansion

```
X_4_a0, log_4_a0, avg_log_4_a0 = gradient_expansion(max_order=4, with_a0=True, igorder=1, ndim=3)
avg_log_4_a0low = integrate_by_parts(pick_a0(avg_log_4_a0))
```

$$\begin{aligned}
&\texttt{avg_log_4_a0low} = C_{010}a_0 + \Lambda a_0 + \left(-\tfrac{1}{2}i + \left(-\tfrac{3}{16}i\right)\psi^{-2}\right) a_0a_0 + \left(\tfrac{1}{6}i + \left(\tfrac{1}{16}i\right)\psi^{-2} + \left(-\tfrac{11}{256}i\right)\psi^{-4}\right) a_{0i}a_{0i} + \\
&\left(\tfrac{1}{2}\psi^{-1}\right)\Lambda a_0a_0 + \left(\left(-\tfrac{1}{4}i\right)\psi^{-1} + \left(\tfrac{5}{32}i\right)\psi^{-3}\right) a_0a_0a_0 + \left(\left(-\tfrac{1}{4}i\right)\psi^{-1} + \left(\tfrac{1}{32}i\right)\psi^{-3}\right) a_0a_ia_i + \left(-\tfrac{1}{3}i + \left(-\tfrac{1}{8}i\right)\psi^{-2}\right)\Lambda a_ia_{0i} + \\
&\left(\tfrac{1}{3}i + \left(\tfrac{1}{8}i\right)\psi^{-2}\right)\Lambda a_{0i}a_i + \left(\tfrac{1}{24}\psi^{-3}\right)\Lambda a_{0i}a_{0i} + \left(\left(-\tfrac{1}{8}\right)\psi^{-2} + \tfrac{5}{64}\psi^{-4}\right) a_0a_ia_{0i} + \left(\tfrac{1}{8}\psi^{-2} + \left(-\tfrac{5}{64}\right)\psi^{-4}\right) a_0a_{0i}a_i + \\
&\left(\tfrac{1}{2}i + \left(-\tfrac{1}{16}i\right)\psi^{-2}\right)\Lambda a_0\Lambda a_0 + \left(\tfrac{1}{2} + \left(-\tfrac{3}{16}\right)\psi^{-2}\right)\Lambda a_0a_0a_0 + \left(\tfrac{1}{6} + \left(-\tfrac{1}{16}\right)\psi^{-2}\right)\Lambda a_0a_ia_i + \left(\tfrac{1}{6} + \tfrac{3}{16}\psi^{-2}\right)\Lambda a_ia_0a_i + \\
&\left(\tfrac{1}{6} + \left(-\tfrac{1}{16}\right)\psi^{-2}\right)\Lambda a_ia_ia_0 + \left(-\tfrac{1}{8}i + \left(\tfrac{5}{64}i\right)\psi^{-2} + \left(-\tfrac{175}{1024}i\right)\psi^{-4}\right) a_0a_0a_0a_0 + \\
&\left(-\tfrac{1}{6}i + \left(\tfrac{1}{16}i\right)\psi^{-2} + \left(-\tfrac{25}{256}i\right)\psi^{-4}\right) a_0a_0a_ia_i + \left(-\tfrac{1}{12}i + \left(-\tfrac{5}{32}i\right)\psi^{-2} + \left(\tfrac{35}{512}i\right)\psi^{-4}\right) a_0a_ia_0a_i + \\
&\left(\left(-\tfrac{1}{4}i\right)\psi^{-1} + \left(\tfrac{5}{96}i\right)\psi^{-3}\right)\Lambda a_0a_ia_{0i} + \left(\left(\tfrac{1}{4}i\right)\psi^{-1} + \left(-\tfrac{5}{96}i\right)\psi^{-3}\right)\Lambda a_0a_{0i}a_i + \left(\left(-\tfrac{1}{4}i\right)\psi^{-1} + \left(\tfrac{1}{96}i\right)\psi^{-3}\right)\Lambda a_ia_0a_{0i} + \\
&\left(\left(-\tfrac{1}{4}i\right)\psi^{-1} + \left(\tfrac{5}{96}i\right)\psi^{-3}\right)\Lambda a_ia_{0i}a_0 + \left(-\tfrac{1}{6}i + \left(-\tfrac{1}{16}i\right)\psi^{-2} + \left(-\tfrac{5}{256}i\right)\psi^{-4}\right)\Lambda a_{0i}\Lambda a_{0i} + \\
&\left(\left(\tfrac{1}{4}i\right)\psi^{-1} + \left(-\tfrac{1}{96}i\right)\psi^{-3}\right)\Lambda a_{0i}a_0a_i + \left(\left(\tfrac{1}{4}i\right)\psi^{-1} + \left(-\tfrac{5}{96}i\right)\psi^{-3}\right)\Lambda a_{0i}a_ia_0 + \left(\left(\tfrac{1}{4}i\right)\psi^{-1} + \left(\tfrac{3}{32}i\right)\psi^{-3}\right)\Lambda a_0\Lambda a_0a_0 + \\
&\left(\left(-\tfrac{1}{4}i\right)\psi^{-1} + \left(\tfrac{1}{32}i\right)\psi^{-3}\right)\Lambda a_0\Lambda a_ia_i + \left(\left(\tfrac{1}{4}i\right)\psi^{-1} + \left(-\tfrac{1}{32}i\right)\psi^{-3}\right)\Lambda a_0a_i\Lambda a_i + \left(\left(\tfrac{1}{4}i\right)\psi^{-1} + \left(-\tfrac{1}{32}i\right)\psi^{-3}\right)\Lambda a_i\Lambda a_ia_0 + \\
&\left(\tfrac{1}{4}\psi^{-1} + \tfrac{5}{32}\psi^{-3}\right)\Lambda a_0a_0a_0a_0 + \left(\tfrac{1}{24}\psi^{-3}\right)\Lambda a_0a_0a_ia_i + \left(\tfrac{1}{4}\psi^{-1} + \left(-\tfrac{5}{96}\right)\psi^{-3}\right)\Lambda a_0a_ia_0a_i + \left(\tfrac{1}{24}\psi^{-3}\right)\Lambda a_0a_ia_ia_0 + \\
&\left(\tfrac{1}{4}\psi^{-1} + \left(-\tfrac{5}{96}\right)\psi^{-3}\right)\Lambda a_ia_0a_0a_i + \left(\tfrac{1}{4}\psi^{-1} + \left(-\tfrac{5}{96}\right)\psi^{-3}\right)\Lambda a_ia_0a_ia_0 + \left(\tfrac{1}{24}\psi^{-3}\right)\Lambda a_ia_ia_0a_0 + \\
&\left(\tfrac{2}{3} + \tfrac{1}{8}\psi^{-2} + \tfrac{1}{32}\psi^{-4}\right)\Lambda a_0\Lambda a_ia_{0i} + \left(-\tfrac{2}{3} + \left(-\tfrac{1}{8}\right)\psi^{-2} + \left(-\tfrac{1}{32}\right)\psi^{-4}\right)\Lambda a_0\Lambda a_{0i}a_i + \left(-\tfrac{1}{3} + \tfrac{1}{128}\psi^{-4}\right)\Lambda a_0a_i\Lambda a_{0i} + \\
&\left(\tfrac{1}{3} + \left(-\tfrac{1}{128}\right)\psi^{-4}\right)\Lambda a_0a_{0i}\Lambda a_i + \left(-\tfrac{1}{3} + \tfrac{1}{128}\psi^{-4}\right)\Lambda a_i\Lambda a_{0i}a_0 + \left(\tfrac{1}{3} + \left(-\tfrac{1}{128}\right)\psi^{-4}\right)\Lambda a_ia_0\Lambda a_{0i} + \\
&\left(-\tfrac{1}{2} + \tfrac{1}{48}\psi^{-2}\right)\Lambda a_0\Lambda a_0\Lambda a_0 + \left(-\tfrac{1}{2} + \left(-\tfrac{1}{16}\right)\psi^{-2}\right)\Lambda a_0\Lambda a_i\Lambda a_i + \left(\tfrac{1}{2}i + \left(-\tfrac{1}{16}i\right)\psi^{-2} + \left(-\tfrac{25}{256}i\right)\psi^{-4}\right)\Lambda a_0\Lambda a_0a_0a_0 + \\
&\left(\tfrac{1}{6}i + \left(-\tfrac{1}{16}i\right)\psi^{-2} + \left(-\tfrac{7}{256}i\right)\psi^{-4}\right)\Lambda a_0\Lambda a_0a_ia_i + \left(\tfrac{1}{6}i + \left(\tfrac{1}{16}i\right)\psi^{-2} + \left(\tfrac{5}{256}i\right)\psi^{-4}\right)\Lambda a_0\Lambda a_ia_0a_i + \\
&\left(\tfrac{1}{6}i + \left(-\tfrac{1}{16}i\right)\psi^{-2} + \left(-\tfrac{7}{256}i\right)\psi^{-4}\right)\Lambda a_0\Lambda a_ia_ia_0 + \left(\tfrac{1}{4}i + \left(-\tfrac{1}{32}i\right)\psi^{-2} + \left(-\tfrac{25}{512}i\right)\psi^{-4}\right)\Lambda a_0a_0\Lambda a_0a_0 + \\
&\left(\tfrac{1}{6}i + \left(-\tfrac{1}{16}i\right)\psi^{-2} + \left(-\tfrac{7}{256}i\right)\psi^{-4}\right)\Lambda a_0a_0\Lambda a_ia_i + \left(\tfrac{1}{6}i + \left(\tfrac{1}{16}i\right)\psi^{-2} + \left(\tfrac{5}{256}i\right)\psi^{-4}\right)\Lambda a_0a_0a_i\Lambda a_i +
\end{aligned}$$

$$\left(\tfrac{1}{12}i+\left(\tfrac{1}{32}i\right)\psi^{-2}+\left(\tfrac{5}{512}i\right)\psi^{-4}\right)\Lambda a_0a_i\Lambda a_0a_i+\left(\tfrac{1}{6}i+\left(\tfrac{1}{16}i\right)\psi^{-2}+\left(\tfrac{5}{256}i\right)\psi^{-4}\right)\Lambda a_0a_i\Lambda a_ia_0+$$
$$\left(\tfrac{1}{6}i+\left(\tfrac{1}{16}i\right)\psi^{-2}+\left(\tfrac{5}{256}i\right)\psi^{-4}\right)\Lambda a_0a_ia_0\Lambda a_i+\left(\tfrac{1}{6}i+\left(\tfrac{1}{16}i\right)\psi^{-2}+\left(\tfrac{5}{256}i\right)\psi^{-4}\right)\Lambda a_i\Lambda a_ia_0a_0+$$
$$\left(\tfrac{1}{12}i+\left(\tfrac{1}{32}i\right)\psi^{-2}+\left(\tfrac{5}{512}i\right)\psi^{-4}\right)\Lambda a_ia_0\Lambda a_ia_0+\left(\left(\tfrac{1}{4}i\right)\psi^{-1}+\left(-\tfrac{1}{96}i\right)\psi^{-3}\right)\Lambda a_0\Lambda a_i\Lambda a_{0i}+$$
$$\left(\left(-\tfrac{1}{4}i\right)\psi^{-1}+\left(\tfrac{1}{96}i\right)\psi^{-3}\right)\Lambda a_0\Lambda a_{0i}\Lambda a_i+\left(\left(-\tfrac{1}{4}\right)\psi^{-1}+\left(-\tfrac{1}{32}\right)\psi^{-3}\right)\Lambda a_0\Lambda a_0\Lambda a_0a_0+$$
$$\left(\tfrac{1}{2}\psi^{-1}+\left(-\tfrac{1}{48}\right)\psi^{-3}\right)\Lambda a_0\Lambda a_0\Lambda a_ia_i+\left(\left(-\tfrac{1}{4}\right)\psi^{-1}+\tfrac{1}{96}\psi^{-3}\right)\Lambda a_0\Lambda a_0a_i\Lambda a_i+\left(\left(-\tfrac{1}{4}\right)\psi^{-1}+\tfrac{1}{96}\psi^{-3}\right)\Lambda a_0\Lambda a_i\Lambda a_0a_i+$$
$$\left(\left(-\tfrac{1}{4}\right)\psi^{-1}+\tfrac{1}{96}\psi^{-3}\right)\Lambda a_0\Lambda a_i\Lambda a_ia_0+\left(\left(-\tfrac{1}{4}\right)\psi^{-1}+\tfrac{1}{96}\psi^{-3}\right)\Lambda a_0\Lambda a_ia_0\Lambda a_i+\left(\left(-\tfrac{1}{4}\right)\psi^{-1}+\tfrac{1}{96}\psi^{-3}\right)\Lambda a_0a_0\Lambda a_i\Lambda a_i+$$
$$\left(-\tfrac{5}{8}i+\left(\tfrac{1}{64}i\right)\psi^{-2}+\left(\tfrac{5}{1024}i\right)\psi^{-4}\right)\Lambda a_0\Lambda a_0\Lambda a_0\Lambda a_0+\left(-\tfrac{5}{6}i+\left(-\tfrac{1}{16}i\right)\psi^{-2}+\left(-\tfrac{1}{256}i\right)\psi^{-4}\right)\Lambda a_0\Lambda a_0\Lambda a_i\Lambda a_i+$$
$$\left(-\tfrac{5}{12}i+\left(-\tfrac{1}{32}i\right)\psi^{-2}+\left(-\tfrac{1}{512}i\right)\psi^{-4}\right)\Lambda a_0\Lambda a_i\Lambda a_0\Lambda a_i$$

Similarly as before, we now separate different powers of $\mu$ and $\psi$, and try to transform each of them to covariant form:

**Code 16.**

```
def get_low_mu(expr, psi_order, order):
    @distributive_op
    def pick_order(m, c, algebra):
        a_order = sum(len(v.idx) for v in m if v.letter == "a")
        return [(m, c)] if a_order == order else []
    if psi_order == 0:
        v = pick_order(expr).map_coefficients(
            lambda z: PP(SR(z).taylor(SR(psi), oo, 0)))
    else:
        v = pick_order(expr).map_coefficients(
            lambda z: PP(z).coefficient(psi**psi_order))
    return v, lambda_to_Q(to_covariant_lambda0(v))

c00, low_a_0_0 = get_low_mu(avg_log_4_a0low, 0, 0)
c01, low_a_0_1 = get_low_mu(avg_log_4_a0low, 0, 1)
c02, low_a_0_2 = get_low_mu(avg_log_4_a0low, 0, 2)
c03, low_a_0_3 = get_low_mu(avg_log_4_a0low, 0, 3)
c04, low_a_0_4 = get_low_mu(avg_log_4_a0low, 0, 4)
c10, low_a_1_0 = get_low_mu(avg_log_4_a0low, -1, 0)
c11, low_a_1_1 = get_low_mu(avg_log_4_a0low, -1, 1)
c12, low_a_1_2 = get_low_mu(avg_log_4_a0low, -1, 2)
c13, low_a_1_3 = get_low_mu(avg_log_4_a0low, -1, 3)
c14, low_a_1_4 = get_low_mu(avg_log_4_a0low, -1, 4)

leftovers = to_covariant_lambda0(tr_permute(
    avg_log_4_a0low
    - (c00 + c01 + c02 + c03 + c04)
    - (c10 + c11 + c12 + c13 + c14)/psi
)).map_coefficients(lambda c: PP(SR(c).taylor(SR(psi),oo,1)))
```

$\texttt{low\_a\_0\_0} = 0$
$\texttt{low\_a\_0\_1} = C_{010}a_0 + Qa_0$
$\texttt{low\_a\_0\_2} = \left(-\tfrac{1}{4}i\right)Q_0Q_0$
$\texttt{low\_a\_0\_3} = \left(-\tfrac{1}{6}\right)F_{0i}Q_i+\left(-\tfrac{1}{4}i\right)QQ_iQ_{0i}+\left(-\tfrac{1}{4}i\right)QQ_0Q_{00}$
$\texttt{low\_a\_0\_4} = \tfrac{1}{6}iF_{0i}F_{0i}+\tfrac{1}{2}iQ_{0i}Q_{0i}+\tfrac{1}{4}iQ_{00}Q_{00}+F_{0i}QQ_{0i}+\tfrac{2}{3}F_{0i}Q_0Q_i+\tfrac{1}{3}F_{0i}Q_iQ_0+\left(-\tfrac{5}{16}i\right)Q_0Q_0Q_0Q_0+$
$\left(-\tfrac{5}{12}i\right)Q_0Q_0Q_iQ_i+\left(-\tfrac{5}{24}i\right)Q_0Q_iQ_0Q_i+\left(-\tfrac{1}{6}i\right)F_{0i}QF_{0i}Q$
$\texttt{low\_a\_1\_0} = \psi^{-1}\Big(0\Big)$
$\texttt{low\_a\_1\_1} = \psi^{-1}\Big(0\Big)$
$\texttt{low\_a\_1\_2} = \psi^{-1}\Big(\tfrac{1}{2}Qa_0a_0\Big)$
$\texttt{low\_a\_1\_3} = \psi^{-1}\Big(\left(-\tfrac{1}{4}i\right)Q_0Q_0a_0+\left(-\tfrac{1}{4}i\right)Q_iQ_ia_0\Big)$
$\texttt{low\_a\_1\_4} = \psi^{-1}\Big(\left(-i\right)F_{0i}Q_{0i}+\left(-\tfrac{1}{2}\right)F_{0i}Q_ia_0+\tfrac{1}{8}QQ_{0i}Q_{0i}+\left(-\tfrac{3}{8}\right)Q_0Q_iQ_{0i}+\left(-\tfrac{1}{2}i\right)F_{0i}QQ_0Q_i+$
$\left(-\tfrac{1}{4}i\right)F_{0i}QQ_iQ_0+\left(-\tfrac{3}{4}i\right)QQ_iQ_{0i}a_0+\left(-\tfrac{1}{4}i\right)QQ_0Q_{00}a_0\Big)$
$\mathit{leftovers} = 0.$

## IV. LONGITUDINAL SHIFT

In this section, we consider the longitudinal modes, but only on the long-wavelength saddle-point level, assuming they can be gradient expanded. The resulting saddle-point shift $B_*$ will appear in derivations starting from the Dyson equation.

Writing $Q = T(\Lambda - 2i\tau B)T^{-1}$, with $[\Lambda, B] = 0$, the $\sigma$-model action is

$$S = \frac{i\pi\nu b}{8\tau}\operatorname{Tr} Q^2 - \frac{i}{2}\operatorname{Tr}\ln[G_0^{-1} + \frac{i}{2\tau}Q] \tag{41}$$

$$= \frac{i\pi\nu b}{8\tau}\operatorname{Tr}(\Lambda - 2i\tau B)^2 - \frac{i}{2}\operatorname{Tr}\ln[T^{-1}\otimes G^{-1}\otimes T + \frac{i}{2\tau}(-2i\tau)B] \tag{42}$$

$$= \frac{i\pi\nu b}{8\tau}\operatorname{Tr}(\Lambda - 2i\tau B)^2 + \operatorname{Tr}\ln\mathcal{G}^{-1} + \delta S[B]\,. \tag{43}$$

We have rescaled the $Q$ field so that the uniform saddle-point equation is satisfied with $Q^2 = 1$; this introduced the scaling factor $b = \tilde{C}(0,1,1)$. Here, $\delta S[B]$ is defined by the same expansion of $\operatorname{Tr}\ln$ as above, with $Q^2 = 1$ assumed, but with $A_0 \mapsto A_0 + TBT^{-1}$, i.e.

$$\delta S[B] = \delta S[a_0 \mapsto a_0 + B] =: \delta S[0] - \frac{\pi\nu}{2}\operatorname{Tr}\big[\tilde{C}(0,1,0)B + \tilde{C}(0,1,1)\Lambda B + \zeta[B]\big] = \delta S[0] + \frac{i\pi\nu}{8\tau}\operatorname{Tr}[4i\tau b\Lambda B + 4i\tau\zeta[B]]\,, \tag{44}$$

and nothing else changes. Here, we have separated out some leading terms in the expansion, with the remainder being in $\zeta$. The diverging constant $C_{010}$ drops out since $\operatorname{tr} B = 0$.

Hence,

$$S = S|_{B=0} + \frac{i\pi\nu}{8\tau}\operatorname{Tr}[-4b\tau^2 B^2 + 4i\tau\zeta[B]] = S|_{B=0} - \frac{\pi\nu}{2}\operatorname{Tr}[ib\tau B^2 + \zeta[B]]\,. \tag{45}$$

Note the leading $\Lambda$-term cancels exactly, due to the rescaling

Let us then find the saddle-point $B_*$. Then,

$$0 = \frac{-\pi\nu}{2}\operatorname{Tr}[(2ib\tau B_* + \frac{\delta\zeta}{\delta B}|_{B_*})\delta B]\,. \tag{46}$$

Now, since $[\delta B, \Lambda] = 0$ we can write it as $\delta B = \frac{1}{2}[(\delta B') + \Lambda(\delta B')\Lambda] = \hat{P}_+(\delta B')$ where $\delta B'$ is an unrestricted matrix. Then we find the saddle-point equation

$$-2ib\tau B_* = \hat{P}_+\frac{\delta\zeta}{\delta B}|_{B_*}\,,\quad \hat{P}_\pm Z := \frac{1}{2}(Z \pm \Lambda Z\Lambda)\,. \tag{47}$$

Substituting it back in, we find the saddle-point level correction,

$$S_B \equiv S|_{B_*} - S|_{B=0} \simeq \frac{i\pi\nu}{8\tau}\frac{1}{b}\operatorname{Tr}\big[(2ib\tau B_*)^2 b + 4ib\tau B_*\frac{\delta\zeta}{\delta B}|_{B_*} + 4ib\tau\tilde{\zeta}[B_*]\big]\,,\qquad \tilde{\zeta}[B] = \zeta[B] - B\frac{\delta\zeta}{\delta B}\,, \tag{48}$$

$$= \frac{i\pi\nu}{8\tau}\frac{1}{b}\operatorname{Tr}\big[2ib\tau B_*\Big(2ib\tau B_* - 4ib\tau B_* + 2\hat{P}_-\frac{\delta\zeta}{\delta B}|_{B_*}\Big)\big] - \frac{\pi\nu}{2}\operatorname{Tr}\tilde{\zeta}[B_*] \tag{49}$$

$$= -\frac{i\pi\nu}{8\tau}\frac{1}{b}\operatorname{Tr}\big(\hat{P}_+\frac{\delta\zeta}{\delta B}|_{B_*}\big)^2 - \frac{\pi\nu}{2}\operatorname{Tr}\tilde{\zeta}[B_*] = \frac{i\pi\nu}{2}b\tau\operatorname{Tr}(B_*)^2 - \frac{\pi\nu}{2}\operatorname{Tr}\tilde{\zeta}[B_*]\,, \tag{50}$$

Here note that $\operatorname{Tr}[(\hat{P}_+Z)(\hat{P}_-Z)] = 0$ and that $\tilde{\zeta}$ has no terms linear in $B$.

To evaluate $S_B$ to fourth order gradients ($\ell^4$) and to $1/\psi^1$, it is sufficient to know $B_*$ up to third order in gradients and to $1/\psi^1$, because we find its leading terms are $\ell^2$ and $\ell/\psi$.

### A. Computer algebra

We can evaluate the above with computer algebra. First, we'll only work in order $1/psi$ and limited gradient order:

**Code 17.**

```
# Define p = 1/psi, and consider only orders 1/psi^0 and 1/psi^1

def PP_psi(order=2):
    """Polynomials in p with p^order = 0"""
    base = PolynomialRing(QQi, 'p')
    p, = base.gens()
    return base.quotient(base.ideal(p**order), names='p')

FF_psi = GG.algebra(PP_psi())

def to_FF_psi(expr):
    return coerce_algebra(expr.map_coefficients(lambda z: z.subs({psi:1/p})), FF_psi)

def from_FF_psi(expr):
    return coerce_algebra(expr, FF).map_coefficients(lambda z: z.subs({p:1/psi}))

def drop_high_psi(expr):
    return from_FF_psi(to_FF_psi(expr))

@distributive_op
def drop_high_a(m, c, algebra, order=4):
    acount = sum(len(v.idx) for v in m)
    return [(m, c)] if acount <= order else []
```

Let us then evaluate the $a_0$ dependent part of $\delta S$, excluding two leading terms:

**Code 18.**

```
zeta_2 = drop_high_a(drop_high_psi(integrate_by_parts(tr_permute(
    pick_a0(avg_log_2_a0) - C_010 * a("0") - PP(C_tilde(0,1,1,order=1,ndim=3)[0]) * Lambda * a("0")))))
zeta_4 = drop_high_a(drop_high_psi(integrate_by_parts(tr_permute(
    pick_a0(avg_log_4_a0) - C_010 * a("0") - PP(C_tilde(0,1,1,order=1,ndim=3)[0]) * Lambda * a("0")))))
```

And then calculate the variation in $a_0$

**Code 19.**

```
@distributive_op
def vary_a0(m, c, algebra):
    res = algebra(0)
    for j, (letter, idx) in enumerate(m.value):
        if letter == "a" and "0" in idx:
            assert idx[0] == "0"
            assert "0" not in idx[1:]
            trailing = idx[1:]
            z = algebra.term(GG(m.value[j+1:] + m.value[:j]), c)
            z = (-1)**len(trailing) * deriv_R(z, trailing[::-1])
            res += z
    return res

dzeta_2_da0 = vary_a0(zeta_2)
dzeta_4_da0 = vary_a0(zeta_4)
```

Then, we calculate the $\hat{P}_+ Z = \frac{1}{2}(Z + \Lambda Z \Lambda)$ projection:

**Code 20.**

```
P_plus_proj = lambda Z: 1/2 * (Z + Lambda * Z * Lambda)

dzeta_2_da0_proj = P_plus_proj(dzeta_2_da0)
dzeta_4_da0_proj = P_plus_proj(dzeta_4_da0)

inv_b = PP((1 / C_tilde(0,1,1,order=4,ndim=3)[0]).taylor(SR.var("psi"), oo, 1))
```

Also covariant form:

**Code 21.**

```
def to_covariant_lambda0_nocycle(expr, max_deg=None, disp=False):
    ideal = lambda0_ideal()
    return reduce_term(expr, ideal, _max_key_lambda0, max_deg=max_deg, disp=disp,
                       simplify=relabel, divide=divide_monomial)
```

We get (truncated to order 2 in gradients):

$$\frac{i}{2b}\hat{P}_+\frac{\delta\zeta}{\delta a_0} = \left(\left(-\tfrac{1}{4}\right)\psi^{-1}\right)Q_0 + \left(\left(\tfrac{1}{2}i\right)\psi^{-1}\right)\Lambda a_0 + \left(\tfrac{1}{8}\psi^{-1}\right)Q_0Q_0 + \left(\tfrac{1}{8}\psi^{-1}\right)Q_iQ_i + \tfrac{1}{4}i\Lambda Q_0Q_0 + \tfrac{1}{12}i\Lambda Q_iQ_i\,. \tag{51}$$

Recall that notation here is with dimensionless gradients, as explained in Sec. III.B. Note the result is order 2 in gradients on $1/\psi^0$ level, and order 1 in gradients on $1/\psi^1$ level.

The saddle-point equation is

$$\tau B_* = f(B_*) = \frac{i}{2b}\hat{P}_+\frac{\delta\zeta}{\delta a_0}|_{a_0\mapsto a_0+B_*}\,. \tag{52}$$

The gradient expansion for $B_*$ can be found by iterating the equation, $B = f(f(\ldots f(B)\ldots))$, until $B$ no longer appears on the RHS in the desired order of gradients and $1/\psi$. In the truncation, we count $B$ to be of order 1 in gradients — this is correct if the final result for $B_*$ is so, and occurs here because there are no $1/\psi^0$ gradient order 0 terms in Eq. (51). The leading terms are given directly by Eq. (51), i.e. gradient order 2 at $1/\psi^0$ and order 1 at $1/\psi^1$. The term of gradient order 2 at $1/\psi^1$ in Eq. (51) needs the iteration to compute.

Let us do this, even though we expect the leading terms come right without iteration,

**Code 22** (Computing $B_*$).

```
@distributive_op
def FF_subs(m, c, algebra, x, y, drop_y=None, drop=None, order=4, disp=False, check=True):
    """Substitute x -> y, with relabeling, dropping terms based on grad order"""
    x = GG(x)
    res = c * algebra.one()

    if drop_y is not None:
        y = drop_y(m, c, x, y, order=order)

    # Substitute in
    free_idxs = set(dummy_idxs) - idxset(m, c)[0]
    for v in m:
        if v.letter == x.letter and v.idx[:len(x.idx)] == x.idx:
            yx = relabel(y, idxs=free_idxs, keep=set(x.idx))
```

```
            res *= deriv_R(yx, v.idx[len(x.idx):], check=check)
            free_idxs = free_idxs - idxset_expr(yx)
        else:
            res *= algebra.term(v, 1)

    if drop is not None:
        res = drop(res, order=order)

    if disp:
        print(res)

    return res

def drop_y(m, c, x, y, order):
    if x == GG(B()):
        # Find gradient order of m, and minimum order of y
        acount, bcount = ab_count(m)
        y_min_order = min(sum(ab_count(m2)) for m2, c2 in y)
        if acount + bcount * y_min_order > order:
            return y.parent()(0)

        # Truncate y to suitable order
        y = drop_high_ab(y, order - acount - max(0, bcount - 1))
    else:
        acount = ab_count(m)[0]
        xcount = ab_count(x)[0]
        y = drop_high_a(y, order - acount + xcount)
    return y

def ab_count(m):
    acount = sum(len(v.idx) for v in m)
    bcount = sum(v.letter == "B" for v in m)
    return acount, bcount

@distributive_op
def drop_high_ab(m, c, algebra, order=4):
    acount, bcount = ab_count(m)
    return [(m, c)] if acount + bcount <= order else []

def solve_B_sp(dzeta, order=2):
    FF_subsx = lambda *a, **kw: FF_subs(*a, **kw, drop_y=drop_y,
                                        drop=drop_high_ab, order=order)

    expr = FF_subsx(dzeta, a("0"), a("0") + B())
    expr = drop_high_a(to_FF_psi(expr), order=order)

    # Fixed-point iteration
    while "B" in letters(expr):
        expr = relabel(FF_subsx(expr, B(), expr))

    expr = drop_high_a(expr, order)
    return from_FF_psi(expr)

B_sp = solve_B_sp(I/2 * inv_b * dzeta_4_da0_proj)
B_sp_cov = lambda_to_Q(to_covariant_lambda0_nocycle(B_sp))
```

This procedure yields:

$$B_* = \left(\left(-\tfrac{1}{4}\right)\psi^{-1}\right)Q_0 + \left(\left(\tfrac{1}{2}i\right)\psi^{-1}\right)Qa_0 + \left(\tfrac{1}{12}\psi^{-1}\right)Q_iQ_i + \tfrac{1}{4}iQQ_0Q_0 + \tfrac{1}{12}iQQ_iQ_i\,. \tag{53}$$

Up to order 2 in gradients and level $1/\psi^0$ and order 1 in gradients and level $1/\psi^1$, it coincides with the first iteration, as claimed. In order 2 in gradients, some difference appears in the $1/\psi^1$ terms.

We can also calculate the gradient order 3 terms similarly,

**Code 23.**

```
@distributive_op
def pick_grad_order(m, c, algebra, order):
    term_order = sum(len(v.idx) for v in m)
    return [(m, c)] if term_order == order else []

B_sp_3 = solve_B_sp(I/2 * inv_b * dzeta_4_da0_proj, order=3)
B_sp_3_cov = lambda_to_Q(to_covariant_lambda0_nocycle(B_sp_3))

B_sp_3_cov_0 = B_sp_3_cov.map_coefficients(lambda z: z.constant_coefficient())
B_sp_3_cov_1 = B_sp_3_cov.map_coefficients(lambda z: z.monomial_coefficient(1/psi))
```

$$
\begin{aligned}
B_* = {} & \left[\tfrac{1}{4}iQQ_0Q_0 + \tfrac{1}{12}iQQ_iQ_i\right] + \left[\tfrac{1}{6}iQ_iQ_{0i} + \left(-\tfrac{1}{6}i\right)Q_{0i}Q_i + \tfrac{1}{4}iQ_0Q_{00} + \tfrac{1}{12}iQ_0Q_{ii} + \right.\\
& \left(-\tfrac{1}{4}i\right)Q_{00}Q_0 + \left(-\tfrac{1}{12}i\right)Q_{ii}Q_0 + \left(-\tfrac{1}{12}\right)F_{0i}QQ_i + \tfrac{1}{12}QF_{0i}Q_i + \tfrac{1}{12}QQ_iF_{0i} + \\
& \tfrac{1}{12}Q_iF_{0i}Q + \left(-\tfrac{1}{2}i\right)QQ_0Q_0Q_0 + \left(-\tfrac{1}{6}i\right)QQ_0Q_iQ_i + \left(-\tfrac{1}{6}i\right)QQ_iQ_0Q_i + \\
& \left.\left(-\tfrac{1}{6}i\right)QQ_iQ_iQ_0\right] + \psi^{-1}\left[\left(-\tfrac{1}{4}\right)Q_0 + \tfrac{1}{2}iQa_0\right] + \psi^{-1}\left[\tfrac{1}{12}Q_iQ_i\right] + \psi^{-1}\left[\left(-\tfrac{1}{24}i\right)F_{0i}Q_i + \right.\\
& \tfrac{1}{24}iQ_iF_{0i} + \tfrac{1}{8}Q_0Q_0Q_0 + \left(-\tfrac{1}{48}\right)Q_0Q_iQ_i + \left(-\tfrac{1}{12}\right)Q_iQ_0Q_i + \left(-\tfrac{1}{48}\right)Q_iQ_iQ_0 + \\
& \tfrac{1}{24}QQ_iQ_{0i} + \left(-\tfrac{1}{8}\right)QQ_{0i}Q_i + \tfrac{1}{8}QQ_0Q_{00} + \left(-\tfrac{1}{24}\right)QQ_0Q_{ii} + \tfrac{1}{8}QQ_{00}Q_0 + \\
& \left.\tfrac{1}{24}QQ_{ii}Q_0 + \left(-\tfrac{1}{4}i\right)QQ_0Q_0a_0 + \tfrac{1}{12}iQQ_iQ_ia_0 + \tfrac{1}{24}iQF_{0i}QQ_i + \tfrac{1}{24}iQQ_iF_{0i}Q\right].
\end{aligned}
\tag{54}
$$

It's clear $B_*^2$ is accurate to gradient order 4 and $\psi^{-1}$.
We can then evaluate the correction to the action:

**Code 24** (Computing $S_B$)**.**

```
def zeta_tilde(zeta, B_sp, order=4):
    """Compute Tr[zeta(B_*) - B_* dzeta/dB_*]"""
    FF_subsx = lambda *a, **kw: FF_subs(*a, **kw, drop_y=drop_y,
                                         drop=drop_high_ab, order=order)

    zp1 = FF_subsx(zeta, a("0"), to_FF_psi(a("0")) + B_sp) - zeta
    dzeta = FF_subsx(vary_a0(zeta), a("0"), to_FF_psi(a("0")) + B_sp)
    zp2 = mul_relabel(B_sp, dzeta)
    return drop_high_a(tr_permute(zp1 - zp2))

def get_dS_B_sp(zeta_4, B_sp, inv_b):
    zeta_4 = to_FF_psi(zeta_4)
    B_sp = to_FF_psi(B_sp)
    inv_b = PP_psi()(inv_b.subs({psi:1/p}))

    zeta_tilde_B_sp = zeta_tilde(zeta_4, B_sp)
    dS_B_sp = tr_permute(drop_high_a(
        -I * inv_b * mul_relabel(B_sp, B_sp) + zeta_tilde_B_sp
    , order=4))
    return from_FF_psi(dS_B_sp)

dS_B_sp = get_dS_B_sp(zeta_4, B_sp_3, inv_b)
dS_B_sp_cov = to_covariant_lambda0(dS_B_sp)

dS_B_sp_cov_0 = lambda_to_Q(dS_B_sp_cov.map_coefficients(lambda z: z.constant_coefficient()))
dS_B_sp_cov_1 = lambda_to_Q(dS_B_sp_cov.map_coefficients(lambda z: z.monomial_coefficient(1/psi)))
```

Hence, (again in dimensionless units III.B),

$$S_B = -\frac{\pi\nu}{2}\,\mathrm{Tr}\Big[\tfrac{1}{16} iQ_0Q_0Q_0Q_0 + \tfrac{1}{24} iQ_0Q_0Q_iQ_i + \tfrac{1}{144} iQ_iQ_iQ_jQ_j + \tfrac{1}{\psi}\Big(\tfrac{2}{3} iF_{0i}Q_{0i} + \tfrac{1}{4} iQ_0Q_0a_0 + \tfrac{1}{12} iQ_iQ_ia_0 + \tfrac{1}{3} F_{0i}Q_ia_0 + \left(-\tfrac{1}{24}\right) QQ_{0i}Q_{0i} + \left(-\tfrac{5}{144}\right) QQ_{ij}Q_{ij} + \tfrac{1}{4} Q_0Q_iQ_{0i} + \tfrac{5}{12} iF_{0i}QQ_0Q_i + \tfrac{1}{12} iF_{0i}QQ_iQ_0 + \tfrac{1}{2} iQQ_iQ_{0i}a_0 + \tfrac{1}{2} iQQ_0Q_{00}a_0\Big)\Big]\,. \tag{55}$$

Similar gradient terms appear as from the base expansion. However, the only generated field strength term involves the "0"-component, so that the spin-Hall $F_{ij}QQ_iQ_j$ term stays unchanged.

We can however recall this is only the saddle-point value $S[B_*]$, which also was obtained assuming a gradient expansion in $B$ can be made.

## V. SADDLE-POINT EQUATIONS

We want to calculate variations of $Q$ under $Q^2 = 1$, ie., $\delta_Q Q = [W, Q]$, and variations of vector potentials, $\delta_A Z_{X,i} = [-iW, Z] + \hat{\nabla}_i(\delta_A Z_X)$, $\delta_A Q = 0$.

**Code 25** (Variations).

```
@distributive_op
def DQ(m, c, algebra):
    res = FF(0)
    for k, (letter, idx) in enumerate(m.value):
        if letter == "Q":
            expr = deriv_R(W() * Q() - Q() * W(), idx, covariant=True)
            res += c * FF(m[:k]) * expr * FF(m[k+1:])
    return res

@distributive_op
def DA(m, c, algebra):
    res = FF(0)
    for k, (letter, idx) in enumerate(m.value):
        if letter == "F" and len(idx) == 2:
            # dF_ij = nabla_i A_j - nabla_j A_i
            expr = V(idx[::-1]) - V(idx)
            res += c * FF(m[:k]) * expr * FF(m[k+1:])
        elif idx:
            i = idx[-1]
            Z = algebra(GG([(letter, idx[:-1])]))
            expr = comm(-I*V(i), Z) + deriv_R(DA(Z), i, covariant=True)
            res += c * FF(m[:k]) * expr * FF(m[k+1:])
    return res

def max_key_Wvar(m):
    # Prefer: no gradients on W/V, not many derivatives outside F
    W_badness = max((len(idx) for letter, idx in m.value if letter == "W"), default=0)
    V_badness = max((len(idx) for letter, idx in m.value if letter == "V"), default=0)
    D_count = sum((len(idx) - (2 if letter == "F" else 0)) for letter, idx in m.value)
    Q_unsymcount = sum(1 for letter, idx in m.value if letter == "Q" and idx and ";" not in idx)
    Q_unsympos = sum(pos for pos, (letter, idx) in enumerate(m.value) if letter == "Q" and idx and ";" in idx)
    return (W_badness, V_badness, Q_unsymcount, -Q_unsympos, D_count, m)

def simpl_var(expr, max_key=max_key_Wvar, sym=False, **kw):
    # Reduce to some canonical form
    return reduce_term(integrate_by_parts_all(expr, max_key=max_key_Wvar, covariant=True),
                       Q_ideal(sym=sym), max_key=max_key, **kw)

def drop_front(expr, sym):
    """Drop monomial factor at the beginning"""
```

```
        res = 0
        for m, c in FF(expr):
            if FF(m[0]) == sym:
                res += c * FF(m[1:])
            else:
                raise ValueError(f"Produced a term not starting with {sym}")
        return res
```

To find results in normal state, we want to also do the substituting $Q \mapsto \begin{pmatrix} 1 & 2f \\ 0 & -1 \end{pmatrix}_K$ and taking the Keldysh component of the resulting equation:

**Code 26** (Normal-state substitution).

```
def QNmat(idxs=()):
    if idxs:
        return matrix(FF, [[0, 2*f(idxs)], [0, 0]])
    else:
        return matrix(FF, [[1, 2*f(idxs)], [0, -1]])

def cNmat(factor):
    return matrix(FF, [[factor, 0], [0, factor]])

def nstate_subs(expr, max_key=max_key_Wvar):
    res = cNmat(0)
    for m, c in expr.monomial_coefficients().items():
        res += cNmat(c) * prod(QNmat(v.idx) if v.letter == "Q" else cNmat(v) for v in m)
    return res[0,1]
```

## A. Matrix current

Expressions for the matrix current from the different terms:

```
S_2 = -I/12 * Q("i")*Q("i")
S_40 = avg_log_4_leading_cov
S_41a = I/12*F("ij")*Q()*Q("i")*Q("j")
S_41b = 1/12*Q()*Q("ij")*Q("ij")
assert S_2 == avg_log_2_p_cov
assert S_41a + S_41b == avg_log_4_psi2_cov

J_2 = drop_front(simpl_var(DA(avg_log_2_p_cov)), V("i"))
J_40 = drop_front(simpl_var(DA(S_40)), V("i"))
J_40_sym = drop_front(simpl_var(DA(S_40), sym=True), V("i"))
J_4a = drop_front(simpl_var(DA(S_41a)), V("i"))
J_4b = drop_front(simpl_var(DA(S_41b)), V("i"))
```

$$\frac{\delta S_2}{\delta A_i} = \left(-\tfrac{1}{3}\right) QQ_i \quad , \tag{56}$$

$$\frac{\delta S_{4,0}}{\delta A_i} = \left(-\tfrac{1}{5}\right) QQ_{(ijj)} + \left(-\tfrac{1}{10}\right) QQ_{(i}Q_jQ_{j)} + \left(-\tfrac{1}{5}\right) QQ_{(i}Q_{jj)}Q + \left(-\tfrac{2}{5}\right) QQ_{(ij}Q_{j)}Q \quad , \tag{57}$$

$$\frac{\delta S_{4,1,a}}{\delta A_i} = \tfrac{1}{12} iQ_{ijj} + \left(-\tfrac{1}{12}\right) F_{ij}Q_j + \left(-\tfrac{1}{12}\right) Q_jF_{ij} + \tfrac{1}{12} iQQ_{ij}Q_j + \tfrac{1}{12} iQ_jQ_{ij}Q + \left(-\tfrac{1}{6} i\right) Q_{ij}QQ_j + \tfrac{1}{12} iQQ_iQ_{jj} + \tfrac{1}{12} iQ_iQ_{jj}Q + \tfrac{1}{12} iQQ_{ijj}Q + \left(-\tfrac{1}{12}\right) QF_{ij}QQ_j + \tfrac{1}{12} QQ_jF_{ij}Q \quad , \tag{58}$$

$$\frac{\delta S_{4,1,b}}{\delta A_i} = \tfrac{1}{6} iQQ_jQ_{ij} + \tfrac{1}{6} iQQ_{ij}Q_j + \left(-\tfrac{1}{6} i\right) Q_jQ_{ij}Q + \tfrac{1}{6} iQ_{ij}QQ_j \quad , \tag{59}$$

We can check $J_{4a}$ has the form claimed in the main text:

```
sage: J_4a_mt = 1/12*(-acomm(F("ij")+Q()*F("ij")*Q(),Q("j"))
....:             + I*deriv_R(Q()*comm(Q("i"),Q("j")),"j",covariant=True))
```

```
sage: reduce_term(V("i")*(J_4a - J_4a_mt), Q_ideal())
```

$$0$$

The torque terms are *defined* as the difference

$$\mathcal{T} = \hat{\nabla}_i J_i - i\frac{\delta S_{\text{grad}}}{\delta Q}\,, \tag{60}$$

where $S_{\text{grad}}$ is the part of the action containing any covariant spatial gradients. We find:

```
get_T = lambda J, S: simpl_var(W()*deriv_R(J, "i", covariant=True) - I*DQ(S))

T_2 = get_T(J_2, S_2)
T_40 = get_T(J_40, S_40)
T_4a = get_T(J_4a, S_41a)
T_4b = get_T(J_4b, S_41b)
```

$$\mathcal{T}_2 = 0\,, \qquad \mathcal{T}_{4a} = 0\,, \qquad \mathcal{T}_{4b} = 0\,, \tag{61}$$

$$\mathcal{T}_{40} = 0\,. \tag{62}$$

**Appendix A: Indexed letter monoid**

**Code 27** (indexed_letter_monoid.py).

```
from sage.structure.all import Parent, UniqueRepresentation, ElementWrapper
from sage.categories.monoids import Monoids
from sage.misc.all import cached_method, sage_wraps
from sage.rings.all import QQ
from sage.structure.richcmp import richcmp, op_EQ, op_NE

class IndexedLetterMonoid(UniqueRepresentation, Parent):
    """
    Noncommutative monomial of indexed letters, and special commutative delta_ij symbol
    """
    def __init__(self, latex_names=None, letter_init=None, letter_weight=None,
                 dummy_idxs=None, extra_idxs=None):
        if dummy_idxs is None:
            dummy_idxs = "ijklmnopqrstuvwxyzabcdefgh"

        if extra_idxs is None:
```

```
            extra_idxs = "0"

        if latex_names is None:
            latex_names = {}

        if letter_init is None:
            letter_init = {}

        if letter_weight is None:
            letter_weight = {}

        letter_init_name = {'involution': self.letter_involution,
                            'symmetric': self.letter_symmetric,
                            'symmetric-tail': self.letter_symmetric_tail,
                            '1-idx': self.letter_at_least_one_idx,
                            '2-idx': self.letter_at_least_two_idx}

        letter_init = dict(letter_init)
        letter_init = {a: letter_init_name[b] if isinstance(b, str) else b
                       for a, b in letter_init.items()}

        self.dummy_idxs = tuple(dummy_idxs)
        self.idxs = self.dummy_idxs + tuple(extra_idxs)
        self.letter_init = letter_init
        self.letter_weight = dict(letter_weight)
        self.latex_names = dict(latex_names)

        Parent.__init__(self, category=Monoids())

    def product(self, x, y):
        return self(x.value + y.value)

    @cached_method
    def one(self):
        return self([])

    @cached_method
    def an_element(self):
        return self.one()

    def _element_constructor_(self, value):
        value = self._from_algebra(value)  # for convenience
        res = []
        res_delta = []
        idx_map = {}
        extra_idx = set()
        main_idx = set()

        for letter, idx in value:
            # Deal with Kronecker deltas first, and reassign indices
            if letter == "delta":
                if len(idx) != 2: raise ValueError(f"invalid delta symbol: {idx!r}")
                idx = sorted(idx_map.get(i, i) for i in idx)
                if idx[1] not in self.dummy_idxs and idx[0] in self.dummy_idxs:
                    idx = self.idxs[::-1]
                if idx[0] == idx[1] and idx[0] in self.dummy_idxs:
                    # We'll keep delta_ii only if the index doesn't appear elsewhere
                    extra_idx.add(idx[0])
                    continue
                main_idx.update(idx)
                res_delta.append((letter, tuple(idx)))
                if idx[1] in self.dummy_idxs:
```

```
                idx_map[idx[1]] = idx[0]

        for letter, idx in value:
            if not all((x in self.idxs or x == ";") for x in idx):
                raise ValueError(f"invalid␣monomial␣index␣({letter!r},␣{idx!r})")

            if letter == "delta":
                continue

            idx = tuple(idx_map.get(i, i) for i in idx)
            if ";" in idx:
                if idx[0] != ";":
                    raise ValueError("Partitioned␣symmetric␣indices␣must␣start␣with␣;")
                if idx == (";",):
                    idx = ()
                else:
                    idx = self.letter_symmetric(res, letter, idx)

            init = self.letter_init.get(letter)
            if init is not None:
                idx = init(res, letter, idx)
                if idx is None:
                    continue

            main_idx.update(idx)
            res.append((letter, idx))

        for i in extra_idx.difference(main_idx):
            res_delta.append(("delta", (i, i)))

        return self.element_class(self, tuple(sorted(res_delta)) + tuple(res))

    def _from_algebra(self, value):
        def _conv(value):
            if hasattr(value, 'monomial_coefficients'):
                # algebra conversion
                (value, c), = value.monomial_coefficients().items()
                if c != 1: raise ValueError("not␣a␣monomial")
            return value
        value = _conv(value)
        value = [_conv(v) for v in value]
        value = [(v.letter, v.idx) if isinstance(v, self.element_class) else v for v in value]
        return value

    class Element(ElementWrapper):
        def _repr_(self, is_latex=False):
            def fmt(part):
                letter, idx = part
                parent = self.parent()
                if is_latex:
                    name = parent.latex_names.get(letter, letter)
                    if ";" in idx:
                        parts = [[]]
                        for i in idx:
                            if i == ";":
                                parts.append([])
                            else:
                                parts[-1].append(i)
                        assert parts[0] == []
                        res = ""
                        for j, ix in enumerate(parts[1:]):
                            ix = "".join(ix)
```

```
                        if j == 0: ix = "(" + ix
                        if j == len(parts) - 2: ix = ix + ")"
                        res += f"{{{name}}}_{{{ix}}}␣"
                    return res
                return f"{{{name}}}" if not idx else f"{{{name}}}_{{{''.join(idx)}}}"
            return letter if not idx else f"{letter}_{''.join(idx)}"
        if not self.value: return "1"
        return "␣".join(map(fmt, self.value))

    def _latex_(self):
        return self._repr_(is_latex=True)

    def _richcmp_(self, other, op):
        # Well-order with finite support:
        # 1. for a nonempty set, there is unique least element,
        # 2. for any m, there are finitely many of m' < m
        if op == op_EQ or op == op_NE:
            return richcmp(self.value, other.value, op)
        a = self._cmp_value(self.value)
        b = self._cmp_value(other.value)
        return richcmp(a, b, op)

    def _cmp_value(self, value):
        # More indices = larger, repeated indices = yet larger, indices on W = largest
        weights = self.parent().letter_weight
        idxord = lambda idx: len(idx) + (len(idx) - len(set(idx)))
        return (len(value),
                max((len(idx) for letter, idx in value), default=0),
                sum(idxord(idx) for letter, idx in value),
                tuple((-weights.get(letter, 0), letter, idxord(idx), idx)
                      for letter, idx in value))

    def __iter__(self):
        return (self.parent()([v]) for v in self.value)

    def __len__(self):
        return len(self.value)

    def __getitem__(self, k):
        return self.parent()(self.value[k] if isinstance(k, slice) else [self.value[k]])

    @property
    def letter(self):
        (letter, idx), = self.value
        return letter

    @property
    def idx(self):
        (letter, idx), = self.value
        return idx

# Letter init methods

@staticmethod
def letter_involution(res, letter, idx):
    if not idx and res and res[-1][0] == letter and not res[-1][1]:
        # letter^2 = 1
        del res[-1]
        return None
    else:
        return idx
```

```
    @staticmethod
    def letter_symmetric(res, letter, idx):
        parts = []
        comma_pos = []
        for j, i in enumerate(idx):
            if i == ";":
                comma_pos.append(j)
            else:
                parts.append(i)

        parts = sorted(parts)

        if comma_pos:
            if comma_pos[0] != 0:
                raise ValueError("Partitioned␣symmetric␣indices␣must␣start␣with␣;")

        for j in comma_pos:
            parts.insert(j, ";")

        return tuple(parts)

    @staticmethod
    def letter_symmetric_tail(res, letter, idx):
        if not idx:
            raise ValueError(f"Index␣for␣{letter}␣must␣have␣at␣least␣1␣entry")
        return (idx[0],) + IndexedLetterMonoid.letter_symmetric(res, letter, idx[1:])

    @staticmethod
    def letter_at_least_one_idx(res, letter, idx):
        if len(idx) < 1:
            raise ValueError(f"Index␣for␣{letter}␣must␣have␣at␣least␣1␣entries")
        return idx

    @staticmethod
    def letter_at_least_two_idx(res, letter, idx):
        if len(idx) < 2:
            raise ValueError(f"Index␣for␣{letter}␣must␣have␣at␣least␣2␣entries")
        return idx

    # Algebra initializer

    def algebra(self, ring, prefix='', bracket=''):
        algebra = super().algebra(ring, prefix=prefix, bracket=bracket)

        def get_constructors(letters):
            constructors = []
            for letter in letters:
                constructors.append(
                    lambda idxs=(), letter=letter: algebra.term(self([(letter, idxs)]),
                                                                algebra.base_ring().one())
                )
            return constructors

        algebra.get_constructors = get_constructors

        return algebra

def distributive_op(func):
    def wrapper(expr, *a, **kw):
        parent = expr.parent()
        if hasattr(parent, 'indices'):
            algebra = parent
```

```
            ring = algebra.base_ring()
        else:
            ring = QQ
            algebra = parent.algebra(ring)
        indices = algebra.indices()
        return parent(algebra.sum_of_terms(
            (indices(m2), ring(c2)) for m, c in algebra(expr)
            for m2, c2 in func(m, c, algebra, *a, **kw)))

    import inspect
    sig = inspect.signature(wrapper)
    wrapper = sage_wraps(func)(wrapper)
    wrapper.__signature__ = sig
    return wrapper

@distributive_op
def relabel(m, c, algebra, idxs=None, keep=(), map=None, swap=False, cmap=None):
    """Relabel dummy indices in *expr*"""
    dummy_idxs = algebra.indices().dummy_idxs
    if idxs is None:
        idxs = dummy_idxs
    ix = []
    if map is None:
        map = {}
    idxs = [i for i in idxs if i not in keep and i not in map and i not in map.values()]
    mvalue = m.value if not swap else m.value[::-1]
    for letter, idx in mvalue:
        ix.extend(j for j in idx if j not in ix and j in dummy_idxs
                  and j not in keep and j not in map)
    if len(ix) > len(idxs): raise ValueError("too few free indices")
    ix_map = dict(zip(ix, idxs))
    ix_map.update(map)
    if cmap is not None:
        c = cmap(c, ix_map)
    p = [(letter, tuple(ix_map.get(j,j) for j in idx)) for letter, idx in m.value]
    return [(p, c)]
```
